# Supplementary material for: Universal Multilayer Network Exploration by Random Walk with Restart
Source: arXiv:2107.04565 ancillary file (2022-10-03)
Supplement: Supplementary file 1 [file MultiXrank_suppmat.pdf]

# Supplementary Information for

## Universal Multilayer Network Exploration by Random Walk with Restart

Anthony Baptista, Aitor Gonzalez and Anaïs Baudot

<sup>1</sup>To whom correspondence should be addressed. E-mail: [anthony.baptista@univ-amu.fr](mailto:anthony.baptista@univ-amu.fr), [anais.baudot@univ-amu.fr](mailto:anais.baudot@univ-amu.fr)

### This PDF file includes:

Figs. S1 to S19  
Tables S1 to S10  
SI References

## Contents

|          |                                                                                                                   |           |
|----------|-------------------------------------------------------------------------------------------------------------------|-----------|
| <b>1</b> | <b>Supplementary information concerning MultiXrank mathematical formulation</b>                                   | <b>3</b>  |
| A        | Proof and rate of convergence                                                                                     | 3         |
| A.1      | Proof of convergence                                                                                              | 3         |
| A.2      | Rate of convergence                                                                                               | 3         |
| B        | Homogeneous exploration                                                                                           | 3         |
| B.1      | Homogeneous parameter: $r$                                                                                        | 4         |
| B.2      | Homogeneous parameter: $\delta$                                                                                   | 4         |
| B.3      | Homogeneous parameter: $\tau$                                                                                     | 4         |
| B.4      | Homogeneous parameter: $\eta$                                                                                     | 4         |
| B.5      | Homogeneous parameter: $\lambda$                                                                                  | 5         |
| C        | Toy model of universal multilayer network (three multiplex networks and three bipartite networks)                 | 5         |
| C.1      | Supra-adjacency matrices of the toy model                                                                         | 5         |
| C.2      | Bipartite network matrices of the toy model                                                                       | 7         |
| C.3      | Random walk with restart (RWR) applied to toy model                                                               | 7         |
| C.4      | Initial probability distribution                                                                                  | 8         |
| C.5      | Normalization of the Supra-heterogeneous adjacency matrix (S)                                                     | 9         |
| D        | Retrieve previous formulas                                                                                        | 10        |
| <b>2</b> | <b>Supplementary information concerning MultiXrank numerical framework</b>                                        | <b>12</b> |
| A        | A hint of time complexity                                                                                         | 12        |
| B        | Input requirements                                                                                                | 13        |
| B.1      | File tree                                                                                                         | 13        |
| B.2      | Networks files                                                                                                    | 14        |
| B.3      | Seeds file                                                                                                        | 14        |
| B.4      | Input parameters file                                                                                             | 14        |
| B.5      | Example for a multilayer network composed of two multiplex networks:                                              | 16        |
| <b>3</b> | <b>Supplementary information concerning the multilayer networks:</b>                                              | <b>17</b> |
| A        | Airport networks                                                                                                  | 17        |
| B        | Biological networks                                                                                               | 18        |
| C        | Hetionet networks                                                                                                 | 18        |
| <b>4</b> | <b>MultiXrank evaluations and Parameter space exploration:</b>                                                    | <b>21</b> |
| A        | Evaluation protocols                                                                                              | 21        |
| A.1      | Leave-One-Out Cross Validation (LOOCV) protocol                                                                   | 21        |
| A.2      | Link Prediction (LP) protocol                                                                                     | 21        |
| A.3      | High connectivity case for RWR on universal multilayer network                                                    | 21        |
| A.4      | Perturbation study of the high connectivity case                                                                  | 22        |
| B        | Exploration of parameter space                                                                                    | 24        |
| <b>5</b> | <b>MultiXrank applications:</b>                                                                                   | <b>31</b> |
| A        | Node Prioritization in Leukemia                                                                                   | 31        |
| B        | Node Prioritization to identify drugs involved in epilepsy and comparison with the Hetionet framework             | 33        |
| C        | Supervised classification of gene-disease associations                                                            | 34        |
| C.1      | Supervised classification protocol                                                                                | 34        |
| C.2      | Comparative analysis of the results obtained from multilayer networks composed of two or three multiplex networks | 38        |

## 1. Supplementary information concerning MultiXrank mathematical formulation

### A. Proof and rate of convergence.

We hypothesize that  $S$  is normalized in a way that makes it a Stochastic matrix.  
We recall that the radius of convergence is defined as follows:

$$R = \sup\{|z| : z \in \mathbb{C}, \sum a_n z^n \text{ converge}\}$$

#### A.1. Proof of convergence.

$p_t = \lambda S p_{t-1} + b$   
 $R(S) = 1$ ; because  $S$  is a Stochastic matrix  
 $R(\lambda S) < 1$ ;  $\lambda \in [0, 1[$  ( $\square$ )  
 So  $\exists p^*, p_t \xrightarrow[t \rightarrow \infty]{} p_*$

#### Proof of ( $\square$ ):

$R(S) = \max(|\lambda_i|)$ ,  $\lambda_i$  = eigenvalue of  $S$   
 So  $R(\lambda S) = \lambda \max(|\lambda_i|)$   
 i.e  $R(\lambda S) = \max(|\lambda \lambda_i|)$ , because  $\lambda_i \in [0, 1]$  (Perron-Frobenius)  
 Thus if  $\lambda \in [0, 1], 0 < R(\lambda S) < R(S) = 1$   
 In conclusion  $R(\lambda S) < 1$

#### A.2. Rate of convergence.

$Ax = b$   
 Let define:  $A = M - N$  and  $H = M^{-1}N$   
 So:  $x = Hx + d \quad \rightarrow \quad x(t) = Hx(t-1) + d$

The spectrum of  $H$  is equal to:  
 $\sigma(H) = \{\lambda_1, \lambda_2, \dots, \lambda_s\}$  and  $1 > |\lambda_1| > \dots > |\lambda_s|$  (Perron-Frobenius)

We define the error at the  $k^{th}$  step as:

$$\begin{aligned} \epsilon(k) &= x(k) - x^* \\ \epsilon(k) &= Hx(k-1) + d - x^* \\ \text{Moreover: } x^* &= Hx^* + d \\ \text{And: } \epsilon(k-1) &= x(k-1) - x^* \\ \text{So: } \epsilon(k) &= Hx(k-1) + d - Hx^* - d \\ &= H(x(k-1) - x^*) \\ &= H\epsilon(k-1) \\ &= H^k \epsilon(0) = (\lambda_1^k G_1 + \dots + \lambda_s^k G_s) \epsilon(0) \\ &\approx \lambda_1^k G_1 \epsilon(0) \text{ (In first order)} \end{aligned}$$

with  $G_i$  = Spectral projection occuring in the spectral decomposition, define such that:

$$G_i = \frac{\prod_{j=1, j \neq i}^k (H - \lambda_j I)}{\prod_{j=1, j \neq i}^k (\lambda_i - \lambda_j)}$$

$$\text{So } \forall i \quad \frac{\epsilon_i(k-1)}{\epsilon_i(k)} \approx \frac{1}{|\lambda_1|}$$

In our case  $\lambda_i = (1 - r)$

In conclusion the rate of convergence at the first order is governed by:  $\frac{1}{(1-r)}$

In other words, the greater  $r$  is, the higher the rate of convergence is. It can be observed in Fig. S4 (see section 2.A).

### B. Homogeneous exploration.

In order to simplify the use of MultiXrank, the user may choose to adopt default parameters. These default parameters are based on three structural properties of the multilayer networks: the number of multiplex networks ( $N$ ), the number of layers in each multiplex network ( $n$ ), and the number of seeds in each multiplex network ( $\alpha$ ).

It is important to note that the number of top nodes (K) given back by MultiXrank is chosen by the user. This parameter K may be an integer between 1 and the total number of nodes, if the user wants to give back all the nodes scored, the variable must be equal to 0.

### B.1. Homogeneous parameter: $r$ .

The parameter  $r$  is associated with the global restart probability. We choose to set this parameter equal to 0.7, which is a value often used in the literature (1).

### B.2. Homogeneous parameter: $\delta$ .

The parameter  $\delta$  is associated with the probability to jump from one layer to another one in a given multiplex network (Fig. 2).

In the case of monoplex network,  $\delta$  is equal to 0, the random walker stays in the layer with probability equal to 1 ( $1-\delta$ ). However, if the random walker is in a multiplex network, the probability is defined as equal to 0.5. In other words, the random walker has the same probability to jump from one layer to another than to stay in the layer. It is to note that  $\delta_i$  corresponds to the  $\delta$  parameter of the multiplex network  $i$  and is equal to 0.5 for each multiplex network, if several multiplex networks are considered.

### B.3. Homogeneous parameter: $\tau$ .

The parameter  $\tau$  is associated with the probability to restart in a specific layer of a multiplex network (Fig. 2). The simplest choice is to choose:  $\tau_{ij} = \frac{1}{n_i} \forall j$ , where  $\tau_{ij}$  represent the probability to restart in the layer  $j$  within the multiplex network  $i$ , and  $n_i$  is the number of layers of the multiplex network  $i$ .

### B.4. Homogeneous parameter: $\eta$ .

The parameter  $\eta$  is associated with the probability to restart in a specific multiplex network (Fig. 2). Let define  $N$  the number of multiplex networks,  $n_i$  the number of layers in the multiplex network  $i$ , and  $\alpha_i$  the number of seeds in the multiplex network  $i$ . It is important to remind that  $\tau_{ij} = \frac{1}{n_i}$  (1). To have a homogeneous exploration the parameter  $\eta$  is constrained by the following equations:

$$\alpha_k \sum_{i=1}^{n_k} \eta_k \tau_{ki} = \alpha_l \sum_{i=1}^{n_l} \eta_l \tau_{li} \quad \forall k, l \quad (2)$$

$$\sum_{j=1}^N \alpha_j [\sum_{i=1}^{n_j} \eta_j \tau_{ji}] = 1 \quad (3)$$

The both equations (2) and (3) can be simplified thanks to (1) as:

$$\alpha_k \eta_k = \alpha_l \eta_l \quad \forall k, l \quad (4)$$

$$\sum_{j=1}^N \alpha_j \eta_j = 1 \quad (5)$$

To solve this set of equations it can be adapted to use an algebraic point of view where it is needed to solve  $X = A^{-1}Y$ , in order to determine  $X = [\eta_1, \eta_2, \dots, \eta_N]^T$ :

$$Y = \begin{pmatrix} 1 \\ 0 \\ \dots \\ 0 \end{pmatrix} ; A = \begin{pmatrix} 1 & 1 & \dots & 1 & 1 \\ \alpha_1 & -\alpha_2 & 0 & \dots & 0 \\ \alpha_1 & 0 & -\alpha_3 & \dots & 0 \\ & & \dots & & \\ \alpha_1 & 0 & \dots & 0 & -\alpha_N \end{pmatrix}$$

It is important to note that if some  $\alpha_i$  terms are equal to zeros, the size of the linear system is reduced to take only the non-zeros  $\alpha_i$  terms.

In other words if there are  $N_s$  non-zeros  $\alpha_i$ , the linear system to solve for the matrix A has a size equal to  $N_s * N_s$ . There are  $N_s$  terms  $\eta_i$  associated with the  $N_s$  non-zeros  $\alpha_i$ , and  $(N - N_s)$  terms  $\eta_i$  associated with zeros  $\alpha_i$  which are equal to zeros.

### B.5. Homogeneous parameter: $\lambda$ .

The parameter  $\lambda$  is associated with the probability to jump from one multiplex network to another one (Fig. 2). Let define  $N$  the number of multiplex networks,  $n_i$  the number of layers in the multiplex network  $i$ , and  $\zeta_i = \frac{1}{n_i}$  the reverse of the number of layers in the multiplex network  $i$ , this variable is defined as a weight to penalize the multiplex networks with several layers, in order to choose a correct  $\lambda_{ij}$  to explore all layers homogeneously. To have a homogeneous exploration, the parameter  $\lambda$  is constrained by the following equations:

$$\sum_{i=1}^N \lambda_{ij} = 1 \quad \forall j \quad (1)$$

$$\zeta_k \lambda_{km} = \zeta_l \lambda_{lm} \quad \forall m, k, l \mid m = k, k \neq l \quad (2)$$

To solve this set of equations it can be adapted to use an algebraic point of view where it is needed to solve  $X = A^{-1}Y$ , in order to determine  $X = [\lambda_{11}, \lambda_{21}, \dots, \lambda_{N1}, \lambda_{12}, \dots, \lambda_{N2}, \lambda_{13}, \dots, \lambda_{1N}, \lambda_{2N}, \dots, \lambda_{NN}]^T$ :

$$Y = \begin{pmatrix} 1 \\ \dots \\ 1 \\ 0 \\ \dots \\ 0 \end{pmatrix}; A = \begin{pmatrix} 1_1 & & & & 0 \\ & 2_1 & & & \\ & & \dots & & \\ & & & 0 & \\ & & & & N_1 \\ \boxed{1_2} & \boxed{0} & \boxed{0} & \dots & \boxed{0} \\ \boxed{0} & \boxed{2_2} & \boxed{0} & \dots & \boxed{0} \\ & & \dots & & \\ \boxed{0} & \boxed{0} & \dots & \boxed{0} & \boxed{N_2} \end{pmatrix}$$

$$\boxed{i_1} = \begin{pmatrix} 1 & 1 & \dots & 1 & 1 \end{pmatrix}; \boxed{i_2} = \begin{pmatrix} -\zeta_1 & 0 & 0 & \dots & 0 & \zeta_i & 0 & \dots & 0 & 0 \\ 0 & -\zeta_2 & 0 & \dots & 0 & \zeta_i & 0 & \dots & 0 & 0 \\ 0 & 0 & -\zeta_3 & \dots & 0 & \zeta_i & 0 & \dots & 0 & 0 \\ & & \dots & & & & & & & \\ 0 & 0 & 0 & \dots & 0 & \zeta_i & 0 & \dots & 0 & -\zeta_N \end{pmatrix}; \boxed{0} = \text{matrix of zero}$$

The size of  $\boxed{i_1}$  is  $1 \times N$ , the size of  $\boxed{i_2}$  and  $\boxed{0}$  is  $(N-1) \times N$ ,  $\forall i \in [1, N]$

The size of  $Y$  is  $N^2$ , there are  $N$  times the value 1 and  $(N-1) \times N$  times the value 0.

It is important to note that  $X$  is a vector with a size equal to  $N^2$  but it is necessary to convert it into a matrix of size  $N \times N$ , because the  $\lambda$  parameter is a  $N \times N$  matrix.

## C. Toy model of universal multilayer network (three multiplex networks and three bipartite networks).

Herein, we propose a full description of a toy model composed of three multiplex networks and their six associated bipartite networks. We detail each matrix and the parameters chosen for the RWR process.

### C.1. Supra-adjacency matrices of the toy model.

Let define:

$A_1$  = Supra-adjacency matrix of the multiplex network 1

$A_1^{[1]}$  = Adjacency matrix of the first layer of multiplex network 1

$A_1^{[2]}$  = Adjacency matrix of the second layer of multiplex network 1

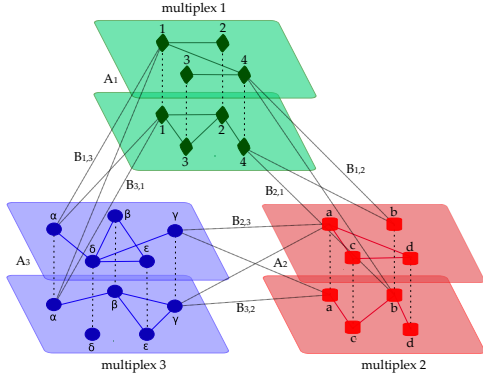

**Fig. S1.** A universal multilayer network composed of three multiplex networks (green, red and blue multiplex networks) and their corresponding Supra-adjacency matrices  $A_i$ , linked by six bipartite networks (represented as bipartite interactions) and their corresponding Bipartite network matrices  $B_{i,j}$ . Note that all the edges can be weighted and/or directed.

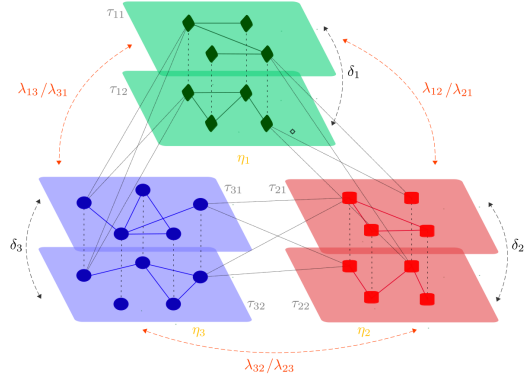

**Fig. S2.** RWR parameters of the toy model composed of three multiplex networks and their associated bipartite networks (represented as bipartite interactions).

### Supra-heterogeneous adjacency matrix

$$\mathcal{S} = \begin{bmatrix} A_1 & B_{1,2} & B_{1,3} \\ B_{2,1} & A_2 & B_{2,3} \\ B_{3,1} & B_{3,2} & A_3 \end{bmatrix}$$

$$p_{t+1}^T = (1-r)\widehat{S}p_t^T + rp_0^T \quad ; \quad \widehat{S} = \text{Normalized } \mathcal{S} \quad [1]$$

### Universal Random Walk with Restart (RWR) equation

- $A_2$  = Supra-adjacency matrix of the multiplex network 2
- $A_2^{[1]}$  = Adjacency matrix of the first layer of multiplex network 2
- $A_2^{[2]}$  = Adjacency matrix of the second layer of multiplex network 2
- $A_3$  = Supra-adjacency matrix of the multiplex network 3
- $A_3^{[1]}$  = Adjacency matrix of the first layer of multiplex network 3
- $A_3^{[2]}$  = Adjacency matrix of the second layer of multiplex network 3
- $I_4$  = Identity matrix in  $M_4(\mathbb{R})$
- $I_5$  = Identity matrix in  $M_5(\mathbb{R})$

$$I_4 = \begin{pmatrix} 1 & 0 & 0 & 0 \\ 0 & 1 & 0 & 0 \\ 0 & 0 & 1 & 0 \\ 0 & 0 & 0 & 1 \end{pmatrix} \quad I_5 = \begin{pmatrix} 1 & 0 & 0 & 0 & 0 \\ 0 & 1 & 0 & 0 & 0 \\ 0 & 0 & 1 & 0 & 0 \\ 0 & 0 & 0 & 1 & 0 \\ 0 & 0 & 0 & 0 & 1 \end{pmatrix} \quad [2]$$

$$A_1 = \begin{bmatrix} A_1^{[1]} & I_4 \\ I_4 & A_1^{[2]} \end{bmatrix} \quad A_1^{[1]} = \begin{pmatrix} 0 & 1 & 0 & 1 \\ 1 & 0 & 0 & 0 \\ 0 & 0 & 0 & 1 \\ 1 & 0 & 1 & 0 \end{pmatrix} \quad A_1^{[2]} = \begin{pmatrix} 0 & 1 & 1 & 0 \\ 1 & 0 & 1 & 1 \\ 1 & 1 & 0 & 0 \\ 0 & 1 & 0 & 0 \end{pmatrix} \quad [3]$$

$$A_2 = \begin{bmatrix} A_2^{[1]} & I_4 \\ I_4 & A_2^{[2]} \end{bmatrix} \quad A_2^{[1]} = \begin{pmatrix} 0 & 0 & 1 & 1 \\ 0 & 0 & 0 & 0 \\ 1 & 0 & 0 & 1 \\ 1 & 0 & 1 & 0 \end{pmatrix} \quad A_2^{[2]} = \begin{pmatrix} 0 & 0 & 1 & 0 \\ 0 & 0 & 1 & 1 \\ 1 & 1 & 0 & 0 \\ 0 & 1 & 0 & 0 \end{pmatrix} \quad [4]$$

$$A_3 = \begin{bmatrix} A_3^{[1]} & I_5 \\ I_5 & A_3^{[2]} \end{bmatrix} \quad A_3^{[1]} = \begin{pmatrix} 0 & 0 & 0 & 1 & 0 \\ 0 & 0 & 0 & 1 & 1 \\ 0 & 0 & 0 & 1 & 0 \\ 1 & 1 & 1 & 0 & 1 \\ 0 & 1 & 0 & 1 & 0 \end{pmatrix} \quad A_3^{[2]} = \begin{pmatrix} 0 & 1 & 0 & 0 & 0 \\ 1 & 0 & 1 & 0 & 1 \\ 0 & 1 & 0 & 0 & 1 \\ 0 & 0 & 0 & 0 & 0 \\ 0 & 1 & 1 & 0 & 0 \end{pmatrix} \quad [5]$$

### C.2. Bipartite network matrices of the toy model.

The bipartite networks are undirected, so the Bipartite network matrices are symmetric:

$$\begin{aligned} B_{2,1} &= B_{1,2}^T \text{ and } b_{2,1} = b_{1,2}^T \\ B_{3,1} &= B_{1,3}^T \text{ and } b_{3,1} = b_{1,3}^T \\ B_{3,2} &= B_{2,3}^T \text{ and } b_{3,2} = b_{2,3}^T \end{aligned}$$

$$B_{1,2} = \begin{bmatrix} b_{1,2} & b_{1,2} \\ b_{1,2} & b_{1,2} \end{bmatrix} \quad b_{1,2} = \begin{pmatrix} 0 & 0 & 0 & 0 \\ 0 & 0 & 0 & 0 \\ 0 & 0 & 0 & 0 \\ 0 & 1 & 0 & 0 \end{pmatrix} \quad [6]$$

$$B_{1,3} = \begin{bmatrix} b_{1,3} & b_{1,3} \\ b_{1,3} & b_{1,3} \end{bmatrix} \quad b_{1,3} = \begin{pmatrix} 1 & 0 & 0 & 0 & 0 \\ 0 & 0 & 0 & 0 & 0 \\ 0 & 0 & 0 & 0 & 0 \\ 0 & 0 & 0 & 0 & 0 \\ 0 & 0 & 0 & 0 & 0 \end{pmatrix} \quad [7]$$

$$B_{2,3} = \begin{bmatrix} b_{2,3} & b_{2,3} \\ b_{2,3} & b_{2,3} \end{bmatrix} \quad b_{2,3} = \begin{pmatrix} 0 & 0 & 1 & 0 & 0 \\ 0 & 0 & 0 & 0 & 0 \\ 0 & 0 & 0 & 0 & 0 \\ 0 & 0 & 0 & 0 & 0 \\ 0 & 0 & 0 & 0 & 0 \end{pmatrix} \quad [8]$$

$$S = \begin{bmatrix} A_1^{[1]} & I_4 & b_{1,2} & b_{1,2} & b_{1,3} & b_{1,3} \\ I_4 & A_1^{[2]} & b_{1,2} & b_{1,2} & b_{1,3} & b_{1,3} \\ b_{2,1} & b_{2,1} & A_2^{[1]} & I_4 & b_{2,3} & b_{2,3} \\ b_{2,1} & b_{2,1} & I_4 & A_2^{[2]} & b_{2,3} & b_{2,3} \\ b_{3,1} & b_{3,1} & b_{3,2} & b_{3,2} & A_3^{[1]} & I_5 \\ b_{3,1} & b_{3,1} & b_{3,2} & b_{3,2} & I_5 & A_3^{[2]} \end{bmatrix} \quad [9]$$

### C.3. Random walk with restart (RWR) applied to toy model.

We include the random walk framework into the Supra-adjacency matrices, to take into account the possibility to jump from one layer to another inside a multiplex network. The parameter  $\delta_i$  control the probability to jump from one layer to another inside the multiplex network  $i$ .

$$A_1 = \begin{bmatrix} (1 - \delta_1)A_1^{[1]} & \delta_1 I_4 \\ \delta_1 I_4 & (1 - \delta_1)A_1^{[2]} \end{bmatrix} \quad [10]$$

$$A_2 = \begin{bmatrix} (1 - \delta_2)A_2^{[1]} & \delta_2 I_4 \\ \delta_2 I_4 & (1 - \delta_2)A_2^{[2]} \end{bmatrix} \quad [11]$$

$$A_3 = \begin{bmatrix} (1 - \delta_3)A_3^{[1]} & \delta_3 I_5 \\ \delta_3 I_5 & (1 - \delta_3)A_3^{[2]} \end{bmatrix} \quad [12]$$

$$S = \begin{bmatrix} (1 - \delta_1)A_1^{[1]} & \delta_1 I_4 & b_{1,2} & b_{1,2} & b_{1,3} & b_{1,3} \\ \delta_1 I_4 & (1 - \delta_1)A_1^{[2]} & b_{1,2} & b_{1,2} & b_{1,3} & b_{1,3} \\ b_{2,1} & b_{2,1} & (1 - \delta_2)A_2^{[1]} & \delta_2 I_4 & b_{2,3} & b_{2,3} \\ b_{2,1} & b_{2,1} & \delta_2 I_4 & (1 - \delta_2)A_2^{[2]} & b_{2,3} & b_{2,3} \\ b_{3,1} & b_{3,1} & b_{3,2} & b_{3,2} & (1 - \delta_3)A_3^{[1]} & \delta_3 I_5 \\ b_{3,1} & b_{3,1} & b_{3,2} & b_{3,2} & \delta_3 I_5 & (1 - \delta_3)A_3^{[2]} \end{bmatrix} \quad [13]$$

#### C.4. Initial probability distribution.

The initial probability distribution  $p_0^T$  is also associated with the restart probability distribution which corresponds to the distribution probability of restarting on specific seeds. So we can write the vector  $p_0^T$  in the general case as follows:

$$p_0^T = \begin{bmatrix} \eta_1 \bar{\mathbf{v}}_0^1 \\ \eta_2 \bar{\mathbf{v}}_0^2 \\ \dots \\ \eta_N \bar{\mathbf{v}}_0^N \end{bmatrix} \quad [14]$$

with  $\eta_i$  the probability to restart in a specific multiplex network  $i$ , and  $\bar{\mathbf{v}}_0^i$  the initial probability distribution of the multiplex network  $i$ , its size equal to  $L_i * m_i$  with  $L_i$  the number of layers of the multiplex network  $i$  and  $m_i$  the number of nodes in the multiplex network  $i$ . We constraint the parameter  $\eta$  with the standard normalization condition that gives that  $\sum_{i=1}^3 \eta_i = 1$ . In our applications, we choose  $\eta_1 = \eta_2 = \eta_3 = 1/3$ , i.e equal probability to restart in each multiplex network.

In the toy model, we choose as seeds the node 1 of multiplex network 1,  $a$  of multiplex network 2, and  $\alpha$  of multiplex network 3. Moreover, we need to add other parameters to take into account the different restart probability in the different layers of each multiplex network. Such parameters are defined as  $\tau$  parameters,  $\tau_{11}$  (resp.  $\tau_{12}$ ) are the probability to restart in the first layer (resp. the second layer) of the first multiplex network,  $\tau_{21}$  (resp.  $\tau_{22}$ ) are the probability to restart in the first layer (resp. the second layer) of the second multiplex network and  $\tau_{31}$  (resp.  $\tau_{32}$ ) are the probability to restart in the first layer (resp. the second layer) of the third multiplex network. So we add the  $\eta$  parameters to  $\bar{\mathbf{v}}_0^i$  such as  $\bar{\mathbf{v}}_0^i = [\tau_{i1}v_0^i, \tau_{i2}v_0^i, \dots, \tau_{in_i}v_0^i]^T$  with  $n_i$  = number of layers in multiplex network  $i$ .

In our application, we choose equal probability to restart in each layer of each multiplex network:

$$\begin{aligned} \tau_{11} &= \tau_{12} = 1/2 \\ \tau_{21} &= \tau_{22} = 1/2 \end{aligned}$$

$$\tau_{31} = \tau_{32} = 1/2$$

Thus,

$$p_0^T = \begin{bmatrix} \eta_1 \bar{\mathbf{v}}_0^1 \\ \eta_2 \bar{\mathbf{v}}_0^2 \\ \eta_3 \bar{\mathbf{v}}_0^3 \end{bmatrix} \quad \bar{\mathbf{v}}_0^1 = \begin{pmatrix} \tau_{11} * 1 \\ 0 \\ 0 \\ 0 \\ \tau_{12} * 1 \\ 0 \\ 0 \\ 0 \end{pmatrix} \quad \bar{\mathbf{v}}_0^2 = \begin{pmatrix} \tau_{21} * 1 \\ 0 \\ 0 \\ 0 \\ \tau_{22} * 1 \\ 0 \\ 0 \\ 0 \end{pmatrix} \quad \bar{\mathbf{v}}_0^3 = \begin{pmatrix} \tau_{31} * 1 \\ 0 \\ 0 \\ 0 \\ \tau_{32} * 1 \\ 0 \\ 0 \\ 0 \end{pmatrix} \quad [15]$$

Finally this initial probability distribution  $p_0^T$  is normalized.

### C.5. Normalization of the Supra-heterogeneous adjacency matrix ( $\mathbf{S}$ ).

The last part concerns the inter-multiplex network parameters  $\lambda$ , which are linked to the normalization of Supra-heterogeneous adjacency matrix, we need to convert it into a Stochastic matrix to ensure the convergence (see section 1.A.1):

$$\hat{\mathbf{S}} = \begin{bmatrix} \hat{S}_{11} & \hat{S}_{12} & \hat{S}_{13} \\ \hat{S}_{21} & \hat{S}_{22} & \hat{S}_{23} \\ \hat{S}_{31} & \hat{S}_{32} & \hat{S}_{33} \end{bmatrix} \quad [16]$$

We will use the formula described below with  $\alpha \in [1, 3]$  and  $\beta \in [1, 3]$ :

$$\hat{S}_{\alpha\alpha}(i_\alpha, j_\alpha) = \begin{cases} \frac{A_\alpha(i_\alpha, j_\alpha)}{\sum_{k_\alpha=1}^{n_\alpha} A_\alpha(i_\alpha, k_\alpha)} & \text{if } \forall \beta : \sum_{k_\beta=1}^{n_\beta} B_{\alpha,\beta}(i_\alpha, k_\beta) = 0 \\ \frac{(1 - \sum_{\beta=1}^c \lambda_{\alpha\beta}) * \lambda_{\alpha\alpha} A_\alpha(i_\alpha, j_\alpha)}{\sum_{k_\alpha=1}^{n_\alpha} A_\alpha(i_\alpha, k_\alpha)} & \text{Otherwise} \end{cases} \quad [17]$$

$$\hat{S}_{\alpha\beta}(i_\alpha, j_\beta) = \begin{cases} \frac{\lambda_{\alpha\beta} B_{\alpha,\beta}(i_\alpha, j_\beta)}{\sum_{k_\beta=1}^{n_\beta} B_{\alpha,\beta}(i_\alpha, k_\beta)} & \text{if } \sum_{k_\beta=1}^{n_\beta} B_{\alpha,\beta}(i_\alpha, k_\beta) \neq 0 \\ \frac{\sum_{\beta=1}^c \lambda_{\alpha\beta} \sum_{i_\alpha=1}^c B_{\alpha,\beta}(i_\alpha, j_\beta)}{\sum_{i_\alpha=1}^c \sum_{k_\beta=1}^{n_\beta} B_{\alpha,\beta}(i_\alpha, k_\beta)} & \text{if } i_\alpha \text{ not in } M_\alpha \\ 0 & \text{Otherwise} \end{cases} \quad [18]$$

So if we describe each term, we obtain:

$$\hat{S}_{11}(i_1, j_1) = \begin{cases} \frac{A_1(i_1, j_1)}{\sum_{k_1=1}^{n_1} A_1(i_1, k_1)} & \text{if } \forall \beta : \sum_{k_\beta=1}^{n_\beta} B_{1,\beta}(i_1, k_\beta) = 0 \\ \frac{(1 - \sum_{\beta=1}^c \lambda_{1\beta}) A_1(i_1, j_1)}{\sum_{k_1=1}^{n_1} A_1(i_1, k_1)} & \text{Otherwise} \end{cases} \quad [19]$$

$$\hat{S}_{22}(i_2, j_2) = \begin{cases} \frac{A_2(i_2, j_2)}{\sum_{k_2=1}^{n_2} A_2(i_2, k_2)} & \text{if } \forall \beta : \sum_{k_\beta=1}^{n_\beta} B_{2,\beta}(i_2, k_\beta) = 0 \\ \frac{(1 - \sum_{\beta=1}^c \lambda_{2\beta}) A_2(i_2, j_2)}{\sum_{k_2=1}^{n_2} A_2(i_2, k_2)} & \text{Otherwise} \end{cases} \quad [20]$$

$$\widehat{S}_{33}(i_3, j_3) = \begin{cases} \frac{\sum_{k_3=1}^{n_3} A_3(i_3, j_3)}{\sum_{k_3=1}^{n_3} A_3(i_3, k_3)} & \text{if } \forall \beta : \sum_{k_\beta=1}^{n_\beta} B_{3,\beta}(i_3, k_\beta) = 0 \\ \frac{(1 - \sum_{\beta=1}^c \lambda_{\alpha\beta}) A_3(i_3, j_3)}{\sum_{k_3=1}^{n_3} A_3(i_3, k_3)} & \text{Otherwise} \end{cases} \quad [21]$$

$$\widehat{S}_{12}(i_1, j_2) = \begin{cases} \frac{\lambda_{12} B_{1,2}(i_1, j_2)}{\sum_{k_2=1}^{n_2} B_{1,2}(i_1, k_2)} & \text{if } \sum_{k_2=1}^{n_2} B_{1,2}(i_1, k_2) \neq 0 \\ 0 & \text{Otherwise} \end{cases} \quad [22]$$

$$\widehat{S}_{13}(i_1, j_3) = \begin{cases} \frac{\lambda_{13} B_{1,3}(i_1, j_3)}{\sum_{k_3=1}^{n_3} B_{1,3}(i_1, k_3)} & \text{if } \sum_{k_3=1}^{n_3} B_{1,3}(i_1, k_3) \neq 0 \\ 0 & \text{Otherwise} \end{cases} \quad [23]$$

$$\widehat{S}_{23}(i_2, j_3) = \begin{cases} \frac{\lambda_{23} B_{2,3}(i_2, j_3)}{\sum_{k_3=1}^{n_3} B_{2,3}(i_2, k_3)} & \text{if } \sum_{k_3=1}^{n_3} B_{2,3}(i_2, k_3) \neq 0 \\ 0 & \text{Otherwise} \end{cases} \quad [24]$$

We computed  $\widehat{S}_{21}$ ,  $\widehat{S}_{23}$ , and  $\widehat{S}_{31}$  with similar formulas.

In this application, we choose an equal probability to jump from one multiplex network to another, or to stay in the same multiplex network.

$$\lambda_{11} = \lambda_{21} = \lambda_{31} = 1/3$$

$$\lambda_{12} = \lambda_{22} = \lambda_{32} = 1/3$$

$$\lambda_{13} = \lambda_{23} = \lambda_{33} = 1/3$$

**Remark :** The equations [17-18] are simplified in the equation [22-24] because the nodes in each bipartite network are also present in the corresponding multiplex network.

#### D. Retrieve previous formulas.

A previous study about RWR on heterogeneous networks has been made by Y.Li et al. (2). The challenging point in this article concerns the Transition rate matrix and more precisely the normalization to obtain it. The normalization is a sine-qua-non condition because without it, the convergence to the steady-state is not assured, see section 1.A.1. Let define  $\mathcal{H}$  the Adjacency matrix of the heterogeneous networks,  $\mathcal{A}_1, \mathcal{A}_2$  the Adjacency matrices of the networks and  $B_{1,2}, B_{2,1}$  the Bipartite network matrices. If the bipartite network is undirected  $B_{2,1} = (B_{1,2})^T$ :

$$\mathcal{H} = \begin{bmatrix} \mathcal{A}_1 & B_{1,2} \\ B_{2,1} & \mathcal{A}_2 \end{bmatrix} \quad [25]$$

As before we can defined the heterogeneous graph  $G_H$  as sets of nodes and edges:

$$\begin{cases} G_H = (V_H, E_H) \\ V_H = \{v_{1,i}, i = 1, \dots, n_1\} \cup \{v_{2,i}, i = 1, \dots, n_2\} \\ E_H = \{e_{i,j}^{1,1}, i, j = 1, \dots, n_1, A_{i,j}^{[1]} \neq 0\} \\ \quad \cup \{e_{i,j}^{2,2}, i, j = 1, \dots, n_2, A_{i,j}^{[2]} \neq 0\} \\ \quad \cup \{e_{i,j}^{1,2}, i = 1, \dots, n_1, j = 1, \dots, n_2, (B_{i,j}^{[1,2]}) \neq 0\} \end{cases} \quad [26]$$

The normalization of this Adjacency matrix, in order to obtain the Transition rate matrix, is based on transformation described in Y.Li et al.

To adopt the same notation as in Y.Li et al., we defined:

$$\alpha = G$$

$$\beta = P$$

$$\lambda = \lambda_{PG} = \lambda_{GP}$$

$$(1 - \lambda) = \lambda_{PP} = \lambda_{GG}$$

$$\begin{aligned}
\hat{S}_{GG} &= M_G \\
\hat{S}_{PP} &= M_P \\
\hat{S}_{GP}(i_G, j_P) &= (M_{GP})_{i,j} \\
\hat{S}_{PG}(i_P, j_G) &= (M_{PG})_{i,j} \\
B_{G,P} &= B \\
B_{P,G} &= B_{G,P}^T = B^T
\end{aligned}$$

We obtain with the previous notation and our general formulation of the normalization the following equations:

$$\hat{S}_{GG}(i_G, j_G) = \begin{cases} \frac{A_G(i_G, j_G)}{\sum_{k_G=1}^{n_G} A_G(i_G, k_G)} & \text{if } \sum_{k_G=1}^{n_G} B_{G,P}(i_G, k_P) = 0 \\ \frac{\lambda_{GG} A_G(i_G, j_G)}{\sum_{k_G=1}^{n_G} A_G(i_G, k_G)} & \text{Otherwise} \end{cases} \quad [27]$$

$$\hat{S}_{PP}(i_P, j_P) = \begin{cases} \frac{A_P(i_P, j_P)}{\sum_{k_P=1}^{n_P} A_P(i_P, k_P)} & \text{if } \sum_{k_P=1}^{n_P} B_{P,G}(i_P, k_G) = 0 \\ \frac{\lambda_{PP} A_P(i_P, j_P)}{\sum_{k_P=1}^{n_P} A_P(i_P, k_P)} & \text{Otherwise} \end{cases} \quad [28]$$

$$\hat{S}_{GP}(i_G, j_P) = \begin{cases} \frac{\lambda_{GP} B_{G,P}(i_G, j_P)}{\sum_{k_P=1}^{n_P} B_{G,P}(i_G, k_P)} & \text{if } \sum_{k_P=1}^{n_P} B_{G,P}(i_G, k_P) \neq 0 \\ 0 & \text{Otherwise} \end{cases} \quad [29]$$

$$\hat{S}_{PG}(i_P, j_G) = \begin{cases} \frac{\lambda_{PG} B_{P,G}(i_P, j_G)}{\sum_{k_G=1}^{n_G} B_{P,G}(i_P, k_G)} & \text{if } \sum_{k_G=1}^{n_G} B_{P,G}(i_P, k_G) \neq 0 \\ 0 & \text{Otherwise} \end{cases} \quad [30]$$

These formulas are the ones obtained in the Li et al. article.

Another study about heterogeneous networks applied RWR to a network composed of a multiplex network and a heterogeneous layer (1). If we choose the same notations as in this article, we retrieve the same formulas.

Overall, our approach can reproduce all the results obtained in previous studies.

## 2. Supplementary information concerning MultiXrank numerical framework

### A. A hint of time complexity.

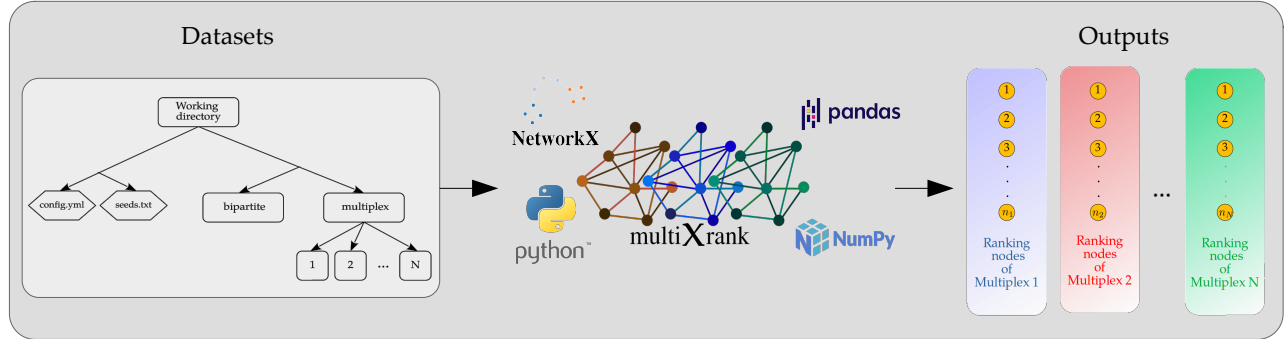

**Fig. S3.** Workflow of the MultiXrank Python package. The networks and the parameters needs to be ordered as in the tree file in the left panel. This tree file is used by MultiXrank to run the RWR on the multilayer network defined in the bipartite and multiplex folders with the parameters given in the config and seeds files. Finally, MultiXrank returns the output scores in an output folder as shown in the right panel. A Conda environment is available on GitHub (<https://github.com/anthbapt/multixrank>) to install all dependencies needed by MultiXrank.

Determining the time complexity of the algorithm depending on the input parameters is an essential point to evaluate the running time. Herein, we just present a hint of MultiXrank complexity. Indeed, some fundamental functions of MultiXrank are based on a high-level Python library, from which the complexity is hard to estimate precisely, thereby, the exact time complexity of MultiXrank is difficult to estimate with precision. Furthermore, we use the standard bounded Landau notation  $O$  to represent the dependence of the function to the input parameters in our code. However, we still give the dependencies on the input parameters that drive the running time of the different functions of MultiXrank class. The most important part concerns the RWR function that computes the Markovian iteration process:

$$p_{i+1}^T = (1 - r)\hat{S}p_i^T + rp_0^T$$

At each iteration, we compute a sparse matrix-vector multiplication and a sum of vectors, until the convergence to the steady-state. These processes have a time complexity of  $O(m)$  and  $O(1)$ , with  $m$  the number of edges in the Transition rate matrix. So this function has a total complexity of  $O(\delta m)$ , where  $\delta$  is the number of iterations.

In conclusion, the time complexity of this part is driven by the number of edges, if the number of nodes is negligible compared to the number of edges, as already described in W.Jin et al. (3).

Then, we compute the average running time over 10 runs for the different functions of the total algorithm. To this goal, we use the multilayer network described in Table S1. The results for the different functions are listed in Table S2, where  $N$  is the number of layers,  $n$  the number of nodes, and  $m$  the number of edges.

So we can see five time-consuming functions: `read_layers`, `get_supra_adj_multiplex`, `get_bipartite`, `get_transition`, and `random_walk_restart`. These five functions represent 98.5% of the running time.

If we make the hypothesis that the number of nodes is negligible compared to the number of edges ( $m \gg n$ ), the total complexity of MultiXrank is  $O\Delta m$ , with  $\Delta$  a constant. So the complexity of MultiXrank is depending on the total number of edges.

#### Remarks:

1. A remaining question concerns the evolution of the running time regarding the input parameters. To partially answer this question, we display the evolution of the running time in function of the global restart probability ( $r$ ) from 0.01 to 0.99. We can see that a correlation exists between MultiXrank running time and the RWR function running time (Fig. S4). This correlation reveals that the global restart parameter ( $r$ ) does not change the running time of the functions, except for the Random Walk with Restart function.
2. Moreover, the running time increases with the inverse of the global restart probability ( $r$ ). This can be explained as the more we decrease the parameter  $r$ , the more we explore the network. This is an expected result given by the proof about the rate of convergence in the section 1.A.2.

| multiplex network | Layer                              | Nodes    | # Interactions |
|-------------------|------------------------------------|----------|----------------|
| 1                 | PPI                                | genes    | 143 653        |
| 1                 | Complexes                          | genes    | 63 561         |
| 1                 | Reactome                           | genes    | 194 500        |
| 2                 | Diseases Similarity                | diseases | 29 200         |
| 3                 | Clinical drug interactions         | drugs    | 14 822         |
| 3                 | Experimental drug interactions     | drugs    | 737            |
| 3                 | Predicted drug interactions        | drugs    | 2 080          |
| 3                 | Pharmacological drugs interactions | drugs    | 48 514         |

| multiplex network | # Nodes |
|-------------------|---------|
| 1                 | 16 947  |
| 2                 | 7 039   |
| 3                 | 1 559   |

| Bipartite networks | # Interactions |
|--------------------|----------------|
| 1-2                | 1 135 037      |
| 2-3                | 1 418 248      |
| 1-3                | 30 895         |

**Table S1.** Networks and parameters chosen to test time complexity

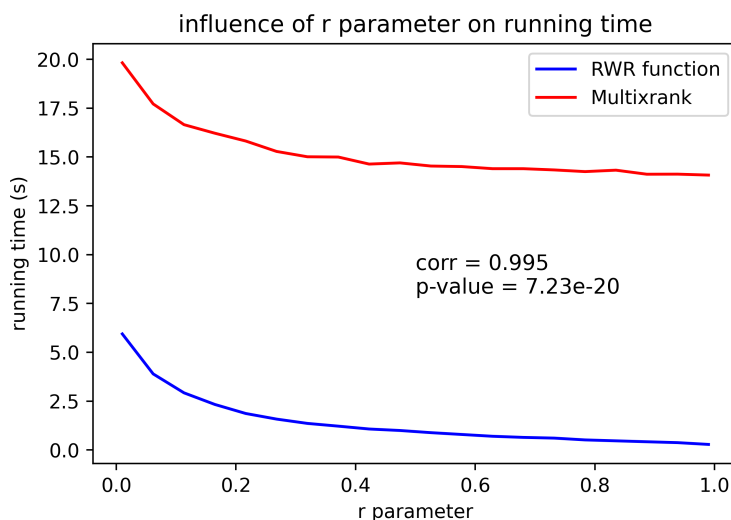

**Fig. S4.** Running time of MultiXrank (red) and of the RWR function (blue) depending on the value of the global restart probability ( $r$ ), the variation of the running time of MultiXrank is correlated (Spearman correlation equal to 0.995) with the running time of the RWR function.

## B. Input requirements.

### B.1. File tree.

To use MultiXrank on universal multilayer networks, one needs to respect a file tree (Fig. S5). The users need to choose a working directory and create two folders and two files. The files are defined as follows: a file dedicated to the input parameters (config.yml) and a second one to the seeds (seeds.txt). The two folders are dedicated to the networks files. The different networks are separated into the bipartite networks folder and the multiplex networks folder.

| Function                  | Running time       | Time complexity                           |
|---------------------------|--------------------|-------------------------------------------|
| multiplex_networks_length | $2.15 * 10^{-6}$ s | $O(1)$                                    |
| check_parameters          | $1.02 * 10^{-3}$ s | $O(1)$                                    |
| read_layers               | $7.40 * 10^{-1}$ s | $O(\delta_1 m)$                           |
| pool_of_nodes             | $9.33 * 10^{-3}$ s | $O(n)$                                    |
| check_seeds               | $7.79 * 10^{-4}$ s | $O(N)$                                    |
| add_missing_nodes         | $2.12 * 10^{-2}$ s | $O(n)$                                    |
| get_number_nodes          | $1.38 * 10^{-4}$ s | $O(N)$                                    |
| get_supra_adj_multiplex   | 1.60 s             | $O(\delta_2 m)$                           |
| get_bipartite             | 6.84 s             | $O(\delta_3 m)$                           |
| get_transition            | 3.96 s             | $O(\delta_4 m)$                           |
| get_seed_scores           | $4.57 * 10^{-3}$ s | $O(N)$                                    |
| random_walk_restart       | $6.55 * 10^{-1}$ s | $O(\delta_5 m)$                           |
| ranking                   | $2.40 * 10^{-1}$ s | $O(n)$                                    |
| top_K_rank                | $6.94 * 10^{-4}$ s | $O(n)$                                    |
| total                     | 14.0 s             | $O(\Delta m + \Gamma n) \sim O(\Delta m)$ |

**Table S2.** Table with the different functions associated with their running time and their hint of time complexity for the multilayer network described in Table S1.

In the multiplex networks folder, the different multiplex networks are associated with different folders, named: 1, 2, ..., N. Inside those folders, the user needs to put all the layers of the multiplex networks with a key-name reported in the input parameters file (config.yml).

In the bipartite networks folder, the user just needs to put all the bipartite networks with a specific name described as follows: NumberOfMultiplexNetwork\_NumberOfOtherMultiplexNetwork.tsv. For example, for a bipartite network between multiplex network 1 and multiplex network 2, the name will be 1\_2.tsv and for the multiplex network 2 and the multiplex network 1, it will be 2\_1.tsv. In the case of a directed bipartite network, both are different. To simplify the creation of the file tree a python script named hierarchy.py is available on Github (<https://github.com/anthbapt/multixrank>). This script creates all the folders needed (for a specific number of multiplex networks) for the running of MultiXrank in a chosen working directory.

### B.2. Networks files.

For the different networks, we use the standard edgelist format, with a tab separation between each column (Fig. S6). The extension used is the TSV, but, every extension with edgelist format can be chosen.

### B.3. Seeds file.

This file contains all the seed nodes. Each row contains one seed, with no preferential order.

### B.4. Input parameters file.

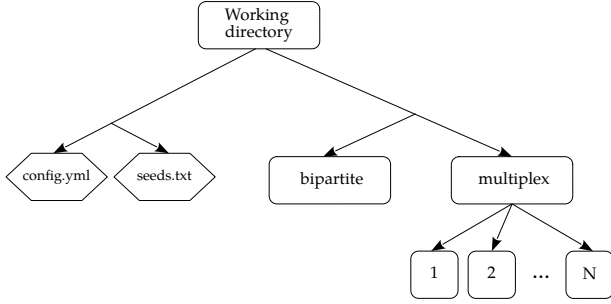

**Fig. S5.** File tree for Networks data and Parameters needed to run MultiXrank.

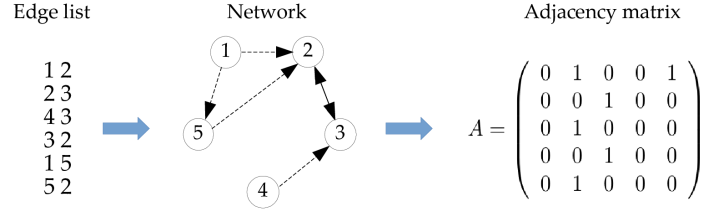

**Fig. S6.** Network file format and representations. The edgelist format is used for MultiXrank to input networks.

We choose YAML format for the input parameters file, to facilitate the import of each parameter into a user-friendly Python type. This file can be divided into two parts. The first one is dedicated to MultiXrank parameters ( $r, \delta, \tau, \lambda, \eta, K$ ), and the second one is dedicated to the network properties parameters that MultiXrank uses.

#### Parameters of the RWR:

- Global restart probability:  $r \rightarrow \text{float}$
- Inter-layer jump probability:  $\delta \rightarrow \text{np.array (1D)}$   
 $\delta_i$  = probability to jump across different layer of the multiplex network  $i$
- Layers restart probability:  $\tau \rightarrow \text{np.array (2D)}$   
 $\tau_{ij}$  = probability to restart in the layer  $j$  of the multiplex network  $i$
- Inter multiplex networks jump probability:  $\lambda \rightarrow \text{np.array (2D)}$   
 $\lambda_{ij}$  = probability to jump from the multiplex network  $i$  to  $j$
- multiplex networks restart probability:  $\eta \rightarrow \text{np.array (1D)}$   
 $\eta_i$  = probability to restart in the multiplex network  $i$
- Number of top nodes:  $K \rightarrow \text{int (0 for all nodes)}$

#### Parameters for the Networks properties:

- seed: Name of the seeds file.
- self\_loops: Boolean value to take into account the self-loops from the network datasets to the network python object. It is preferable to choose self\_loops equal to 0 (without self-loops).
- Multiplex:
  - layers: list of the paths to the layers of the multiplex network considered
  - graph\_type: list of the types of the different layers in the multiplex network considered according to the Table 3.
- Bipartite: list of the information concerning each bipartite network: the source (number of the source multiplex network), the target (number of the target multiplex network), and the type of the bipartite network (graph\_type) according to the Table 3.

#### Notations for the type of interactions:

The notation to precise the different type of interactions in each multiplex network and bipartite network is based on a Boolean code (Table S3) where the first digit is dedicated to the weight and the second one to the directed property.

| name          | directed | weighted | boolean code |
|---------------|----------|----------|--------------|
| undirweighted | 0        | 0        | 00           |
| weighted      | 0        | 1        | 01           |
| directed      | 1        | 0        | 10           |
| dirweighted   | 1        | 1        | 11           |

**Table S3.** Boolean code to precise the kind of interactions (edges) in multiplex networks and in the bipartite networks.

#### B.5. Example for a multilayer network composed of two multiplex networks:.

**Remark:**

If undirected bipartite networks are considered, the Bipartite network matrices are symmetric. The example in Fig. S7 belongs to this case, so Bipartite\_interactions is equivalent to  $[[0, "00"], ["00", 0]]$ .

```
# Name of the seeds file
seed: seeds.txt
# Global Restart Probability (r)
r: 0.7
# Multiplex Networks Restart Probability (eta)
eta: [1/2, 1/2]
# Inter Multiplex Networks Jump Probability (lambda)
lamb:
  - [1/2, 1/2]
  - [1/2, 1/2]

multiplex:
  1:
    layers:
      - multiplex/1/PPI.tsv
      - multiplex/1/Reactome.tsv
      - multiplex/1/Complexes.tsv
    # Inter Layers Jump Probability (delta) : for multiplex 1
    delta: 0.5
    # Graph type: (un)weighted, (un)directed : for multiplex 1
    graph_type: [00, 00, 00]
    # Layers Restart Probability (tau) : for multiplex 1
    tau: [1/3, 1/3, 1/3]
  2:
    layers:
      - multiplex/2/disease_disease_final.tsv
    # Inter Layers Jump Probability (delta) : for multiplex 2
    delta: 0
    # Graph type: (un)weighted, (un)directed : for multiplex 2
    graph_type: [00]
    # Layers Restart Probability (tau) : for multiplex 2
    tau: [1]

bipartite:
  # Bipartite network information
  bipartite/1_2.tsv: {source: 1, 'target': 2, graph_type: 00}
```

**Fig. S7.** Example of input parameters file for multilayer network composed of two multiplex networks (gene and disease networks).

### 3. Supplementary information concerning the multilayer networks:

The different networks described in Table S4 are available on GitHub in edgelist format (<https://github.com/anthbapt/multixrank>).

| System            | # Multiplexes | # Layers in each multiplex | Nodes                                                                                                                     | # Nodes                                                                  | Edges                                                                                                                | # interactions                                                                                                                  | Bipartites                                                                                                                                                  |
|-------------------|---------------|----------------------------|---------------------------------------------------------------------------------------------------------------------------|--------------------------------------------------------------------------|----------------------------------------------------------------------------------------------------------------------|---------------------------------------------------------------------------------------------------------------------------------|-------------------------------------------------------------------------------------------------------------------------------------------------------------|
| Toy model         | 3             | 2, 2, 2                    | \                                                                                                                         | 4 ; 4 ; 5                                                                | \                                                                                                                    | 1 : 7 ; 2 : 6 ; 3 : 9                                                                                                           | 1-2 : 1 ; 1-3 : 1 ;<br>2-3 : 1                                                                                                                              |
| Airport           | 3             | 3, 3, 3                    | French, UK, German Airports                                                                                               | 18 ; 28 ; 23                                                             | Company connections                                                                                                  | 1 : 15, 5, 9<br>2 : 23, 43, 9<br>3 : 41, 35, 12                                                                                 | 1-2 : 51<br>1-3 : 39<br>2-3 : 61                                                                                                                            |
| Biological system | 3             | 3, 1, 4                    | Genes, Diseases, Drugs                                                                                                    | 16 967 ; 7 039 ;<br>1 559                                                | PPI, Complexes, Reactome ;<br>Diseases similarity ;<br>drug1, drug2, drug3, drug4                                    | 1 : 143 653, 63 561,<br>194 500<br>2 : 29 200<br>3 : 14 822 ; 737 ;<br>2 080 ; 48514                                            | 1-2 : 1 135 037<br>1-3 : 30 895<br>2-3 : 1 418 248                                                                                                          |
| Hetionet          | 9             | 3, 1, 1, 1, 1, 1, 1, 1, 1  | Genes, Diseases, Compounds, Anatomy parts, Symptoms, Sides effects, Pharmacologic classes, Pathways, Biological processes | 25 003 ; 136 ;<br>1 538 ; 400 ;<br>415 ; 5 701 ;<br>345 ; 1 822 ; 11 381 | Genes covaries , Genes interactions, Genes regulations ;<br>Diseases similarity ;<br>Coumpounds similarity ;<br>Self | 1 : 61 690, 147 164,<br>265 672<br>2 : 543<br>3 : 6 486<br>4 : self<br>5 : self<br>6 : self<br>7 : self<br>8 : self<br>9 : self | 1-8 : 84 372<br>1-9 : 559 504<br>2-1 : 27 972<br>2-4 : 3 602<br>2-5 : 3 357<br>3-1 : 51 429<br>3-2 : 1 145<br>3-6 : 138 944<br>4-1 : 726 495<br>7-3 : 1 029 |

**Table S4.** Properties of the different networks used in the article.

#### A. Airport networks.

The different multiplex networks were generated from the connections between airports given by data published in Cardillo et al (4). The mapping of the airports to their respective countries has been done thanks to the database <https://openflights.org/data.html>.

The companies were chosen based on their number of connections, we took the top-3 most connected companies for each country.

##### 1. French airports multiplex network:

- **FR3:** Easyjet connections between French airports.
- **FR7:** Air France connections between French airports.
- **FR26:** Netjets connections between French airports.

##### 2. British airports multiplex network:

- **UK3:** Easyjet connections between British airports.
- **UK15:** Flybe connections between British airports.
- **UK26:** Netjets connections between British airports.

##### 3. German airports multiplex network:

- **G1:** Lufthansa connections between German airports.
- **G6:** Air Berlin connections between German airports.
- **G24:** Germanwings connections between German airports.

The bipartite networks correspond to the transnational flights operated by these different companies between France and UK, France and Germany, British and Germany.

## B. Biological networks.

1. **gene multiplex network:** This multiplex network is composed of three different layers of interactions between genes. Please note that we considered genes and proteins indifferently. We choose the gene-name annotation for this multiplex network and its associated bipartite networks.
  - **Complexes:** A molecular complexes layer constructed from the fusion of Hu.map (5) and Corum (6), using OmniPathR (7).
  - **PPI:** Protein-Protein interaction (PPI) layer corresponding to the fusion of 3 datasets: APID (homo sapiens level 2, without inter-species interactions), Hi-Union and Lit-BM ([www.interactome-atlas.org/download](http://www.interactome-atlas.org/download)). It is important to notice that 166 over 13346 apid proteins do not match to any gene-names, so we choose to use the uniprot ID in this case.
  - **Reactome:** A pathways layer extracted from NDEx (8) and corresponding to the human Reactome data (9).
2. **Disease monoplex network:** The networks were built on phenotypic proximity between diseases calculated thanks to the information content. The whole protocol is described in (1). We choose the UMLS annotation for diseases in this monoplex network and its bipartite networks.
3. **Drug multiplex network:** The data used come from Cheng et al (10)<sup>†</sup> and pharmacological drugs interaction network from [snap.stanford.edu](http://snap.stanford.edu)<sup>‡</sup>. We use the drugbank name format for the drugs in this multiplex network and its bipartite networks.
  - **drug1<sup>†</sup>:** Clinical drug interactions (clinically reported adverse drug–drug interactions, 14822 clinically reported adverse drug–drug interactions connecting 667 drugs were retained )
  - **drug2<sup>†</sup>:** Experimental drug combinations (experimentally validated drug combinations, 737 unique pairwise drug combinations connecting 376 drugs were retained)
  - **drug3<sup>†</sup>:** Predicted drug combinations (network-predicted hypertensive drug combinations, 2080 potential combinations involving 65 hypertensive drugs were retained)
  - **drug4<sup>‡</sup>:** Drug-Drug interactions determined from the pharmacologic effect of the action of one drug on another drug (48514 interactions involving 1514 drugs).

Bipartite networks are defined as follows:

- **Gene-Disease (1-2):** The bipartite network come from the 2020 version (v7.0) of DisGeNET (11). This network is weighted with score computed according to the formula reported in <https://www.DisGeNET.org/dbinfo>. It is to note that a 2014 version of the gene-disease association of DisGeNET (v2.0) is used for the training of the binary classifier exposed in the section 5.C.
- **Gene-Drug (1-3):** Several bipartite networks are available: drug-target association from drugBank Release Version 5.1.8 [go.drugbank.com/releases/latest](http://go.drugbank.com/releases/latest), drug-target associations from drugcentral release v10.12 [drugcentral.org/download](http://drugcentral.org/download), and the drug-target association from Cheng et al (10). We merged all of them to obtain our bipartite network.
- **Disease-Drug (2-3):** The disease-drug association network come from repoDB from (12).

It is important to note that some nodes are just present in the bipartite networks. Thus we can added artificially these nodes by adding self-loops in one of the layers of the corresponding multiplex network to take them as specific nodes, and then ranked them with MultiXrank.

## C. Hetionet networks.

Hetionet (13) is composed of heterogeneous networks constructed by integrating knowledge and experimental findings from millions of publications of biomedical research. This heterogeneous network contains nine kinds of nodes: genes, diseases, compounds, anatomy parts, symptoms, side effects, pharmacologic classes, pathways, biological processes. In our formalism, it is necessary to represent the original data suitably for MultiXrank, i.e, multiplex networks (or monoplex networks) and bipartite networks. However, some kind of nodes are just present in the bipartite networks, thus it could be needed to create an artificial self-loop network to take them as specific nodes.

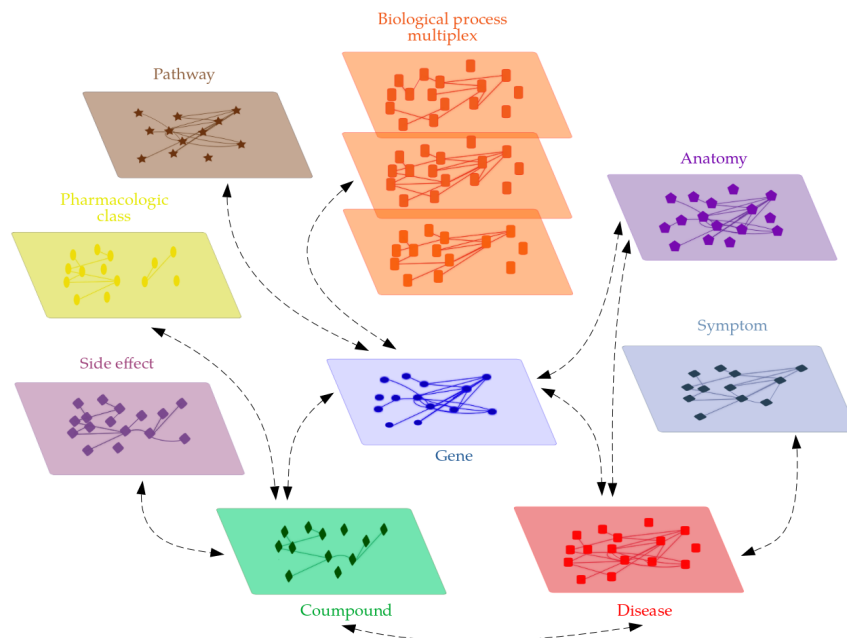

**Fig. S8.** Hetionet heterogeneous network adapted from D.S.Himmelstein et al (13)

1. **gene multiplex network:** Three layers Gene–covaries–Gene (GcG), Gene–interacts–Gene (GiG), Gene–regulates–Gene (GrG)
2. **Disease monoplex network:** Disease–resembles–Disease (DrD)
3. **Compound monoplex network:** Compound–resembles–Compound (CrC)
4. **Anatomy part monoplex network:** The nodes was extracted from bipartite networks 2-4 and 4-1 (self-loops network)
5. **Symptom monoplex network:** The nodes was extracted from bipartite networks 2-5 (self-loops network)
6. **Side effect monoplex network:** The nodes was extracted from bipartite networks 3-6 (self-loops network)
7. **Pharmacologic classe monoplex network:** The nodes was extracted from bipartite networks 7-3 (self-loops network)
8. **Pathway monoplex network:** The nodes was extracted from bipartite networks 1-8 (self-loops network)
9. **Biological processe monoplex network:** The nodes was extracted from bipartite networks 1-9 (self-loops network)

Bipartite networks are defined as follows (For more details see the Table 2 from D.S.Himmelstein et al (13)):

- **Gene-Pathway (1-8):** Gene–participates–Pathway (GpPW)
- **Gene-Biological Process (1-9):** Gene–participates–Biological Process (GpBP)
- **Anatomy Part-Gene (4-1):** Merged of three layers, Anatomy–downregulates–Gene (AdG), Anatomy–expresses–Gene (AeG), Anatomy–upregulates–Gene (AuG)
- **Disease-Anatomy part (2-4):** Disease–localizes–Anatomy (DIA)
- **Disease-Symptom (2-5):** Disease–presents–Symptom (DpS)
- **Compound-Side effect (3-6):** Compound–causes–Side Effect (CcSE)

- **Pharmalogic classes-Compound (7-3):** Pharmacologic Class–includes–Compound (PCiC)
- **Disease-Gene (2-1):** Merged of three layers, Disease–associates–Gene (DaG), Disease–downregulates–Gene (DdG), Disease–upregulates–Gene (DuG)
- **Coumpound-Disease (3-2):** Merged of two layers, Compound–palliates–Disease (CpD), Compound–treats–Disease (CtD)
- **Coumpound-Gene (3-1):** Merged of two layers, Compound–downregulates–Gene (CdG), Compound–upregulates–Gene (CuG)

## 4. MultiXrank evaluations and Parameter space exploration:

### A. Evaluation protocols.

For each validation protocol, we consider a bipartite network that links two kinds of nodes. Herein, we apply the validation on the airports universal multilayer network, considering the bipartite network between the French and the British airports. For the biological universal multilayer network, we consider the bipartite network between gene multiplex network and disease monoplex network. Both multilayer networks are described in section 3.A-B.

To simplify the notation in the following, we will call the two monoplex/multiplex networks linked by the bipartite network: monoplex/multiplex network 1 (M1), the monoplex/multiplex network for which we remove nodes (during the validation protocol described below), and monoplex/multiplex network 2 (M2), the monoplex/multiplex network for the one we want to predict the associations. For example, in the case of the gene-disease associations, the multiplex network 1 is the gene multiplex network, and the multiplex network 2 is the disease monoplex network. In other words, we want to predict genes association for each disease.

#### A.1. Leave-One-Out Cross Validation (LOOCV) protocol.

To evaluate the performances of our framework on different networks, we design a Leave-One-Out Cross-Validation (LOOCV) protocol inspired by F.Mordelet and J.P.Vert (14) and A.Valdeolivas et al. (1). For each node of M2 associated with at least two nodes of M1, we take all the associated M1 nodes. The edges associating the M1 nodes with a given M2 node are removed from the bipartite network one by one, and the corresponding M1 node each time is considered as the left-out M1 node. The remaining M1 nodes associated with the same M2 node are used as seed(s), as well as the M2 node when the M2 network is considered. The RWR algorithms are then applied, and all the network nodes are scored and ranked according to their proximity to the seed(s). The rank of the M1 node that was left-out in the current run is recorded. The process is repeated iteratively for each left-out M1 node. Finally, the Cumulative Distribution Function (CDF) of the ranks of the left-out M1 nodes is plotted (Fig. 3). The CDF displays the percentage of left-out M1 nodes that are ranked within the top-K M1 nodes. The CDFs are used to evaluate and compare the performance of RWR on different combinations of networks: multiplex network, multilayer network composed of two or three monoplex/multiplex networks, and so on.

Leave-one-out cross-validations on monoplex network, and multiplex network networks only used the nodes from M1 as seed(s) for the RWR process.

Leave-one-out cross-validation on heterogeneous, multilayer network composed of two or three monoplex/multiplex networks used nodes from M1, and also the nodes from M2 for the RWR process. It is to note that in order to simulate an unknown association, we also remove the bipartite association linking the left-out M1 node and the M2 node of the current run. Doing so, we avoid the artificial top ranking of the left-out M1 nodes.

It is to note, for the biological multilayer network, we use a subpart of DisGeNET v7.0 (described in section 3.A.2) where we extract only bipartite interactions with a score superior or equal to 0.3 (a threshold that gives us enough associations to obtain a smooth LOOCV curve).

#### A.2. Link Prediction (LP) protocol.

Another way to evaluate the performances of our framework is to use a Link Prediction (LP) protocol. In this case, we used all the associations, including the nodes from M2 associated with one node from M1. We systematically removed associations between M1 nodes and M2 nodes from the corresponding bipartite network, and we predicted the rank of this M1 node using the M2 node as a seed in the RWR.

All the network nodes are scored and ranked according to their proximity to the seed. The rank of the M1 node from the association that was left out in the current run is recorded. Finally, the Cumulative Distribution Function (CDF) of the ranks of the left-out node of M1 is plotted as described just above.

#### A.3. High connectivity case for RWR on universal multilayer network.

When we try to perform validation with standard datasets, adding new multiplex networks may not increase the predictive power. The reason is that the walk from one node to another may not exist or it is a very long path (except for the original bipartite network). For instance, if we take an example from Fig. S10, if we want to predict a removed link between a node from the disease monoplex network to the gene multiplex network, we need to have a connection between neighbor nodes from this both multiplex networks, or if we used information from the third multiplex network, we need to have a short walk from the disease node to the drug multiplex network and then, from the drug multiplex network to the gene multiplex network. So if such a connection does not exist or if it is too long, the third multiplex

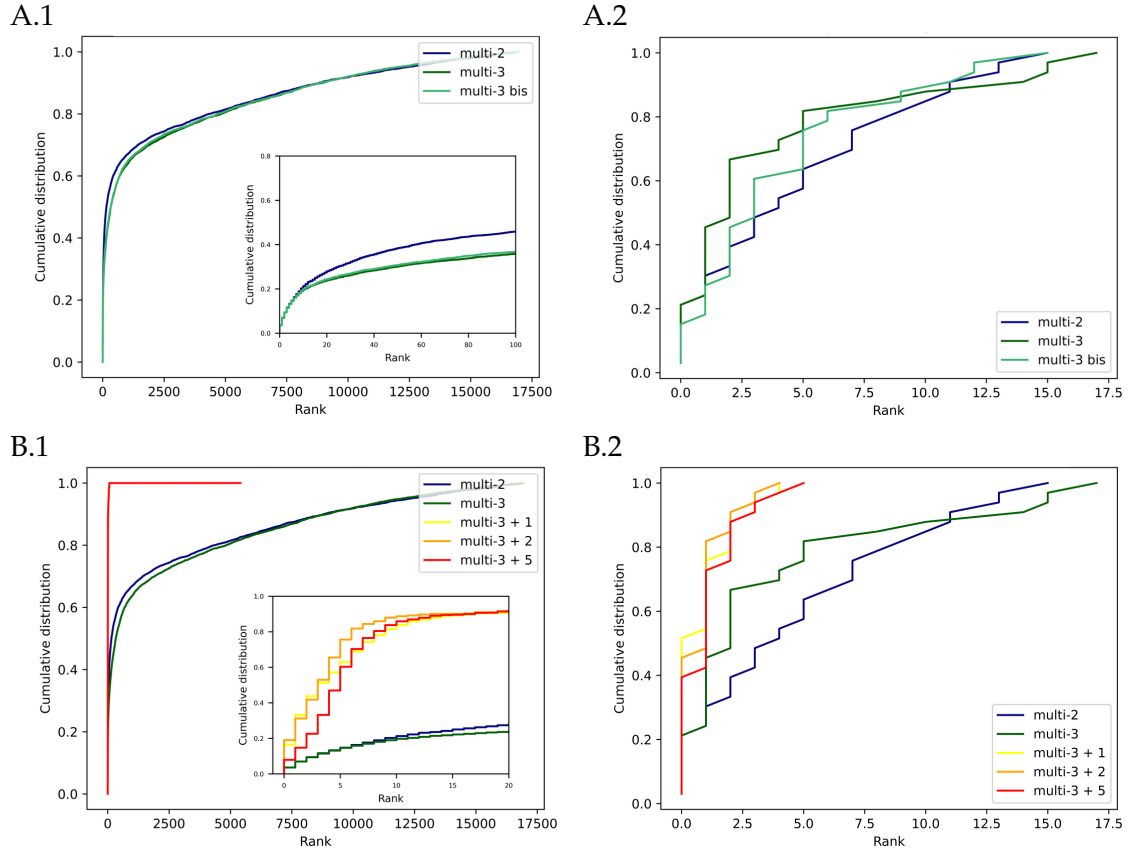

**Fig. S9.** A.1-2: Cumulative Distribution Functions (CDFs) representing the ranks of the left-out nodes for LP protocol. A.1: focus on different combinations of biological networks: the multilayer network composed of gene multiplex network and disease monoplex network (multi-2), and the multilayer network composed of genes, drug multiplex networks and the disease monoplex network for two very different sets of parameters (multi-3, multi-3 bis). A.2: focus on different combinations of airports networks: French and British airports multiplex networks (multi-2), and French, British, and German airports multiplex networks for two different sets of parameters (multi-3, multi-3 bis). All these multiplex networks are connected with the bipartite networks described in Evaluations section.

B.1-2: Cumulative Distribution Functions (CDFs) representing the ranks of the left-out nodes in the LP protocol for the networks described previously with the 3-multiplex networks with artificially increased connectivity in the gene-drug and disease-drug bipartite networks thanks to 1 (multi3+1), 2 (multi3+2) or 5 (multi3+5) transit nodes for each gene-disease association (B.1), and for French-British airports association (B.2).

network does not increase the predictive power. This is similar to the shortest path method where a very long path does not contribute.

When we checked if the genes and disease nodes in the gene-disease bipartite network are also present in the gene-drug and disease-drug bipartite networks we saw that this overlap was very low Fig. S10, that explains why if we used a third drug multiplex network that does not change anything for biological multilayer (LOOCV for Biological multilayer, Fig. S9.A.1). However, we can see an increase in the predictive power for the airport multilayer (Fig. S9.A.2).

To check our postulate we create new bipartite networks between the drug multiplex network (German airports multiplex network) and the gene multiplex network (French airports multiplex network), and between the drug multiplex network (German airports multiplex network) and the disease monoplex network (British airports multiplex network). To do so, we added simulated transit drug nodes linking diseases to genes (German nodes linking British to French airports) to artificially increase the connectivity of the multilayer network (Fig. S11). We show that that these artificially added transit nodes increase drastically the prediction performance for both LOOCV (Fig. 3.B.1-2) and LP (Fig. S9.B.1-2).

#### A.4. Perturbation study of the high connectivity case.

The previous section shows the high connectivity case, however, to confirm that high connected bipartite networks increase the predictive power of the RWR process, we need to check if the reverse process can decrease the predictive power. In other words, if a perturbation of the bipartite networks designed in the previous section (Fig. S11) changes the predictive power. To do so, we shuffled the nodes in bipartite networks; this is similar to use random networks as

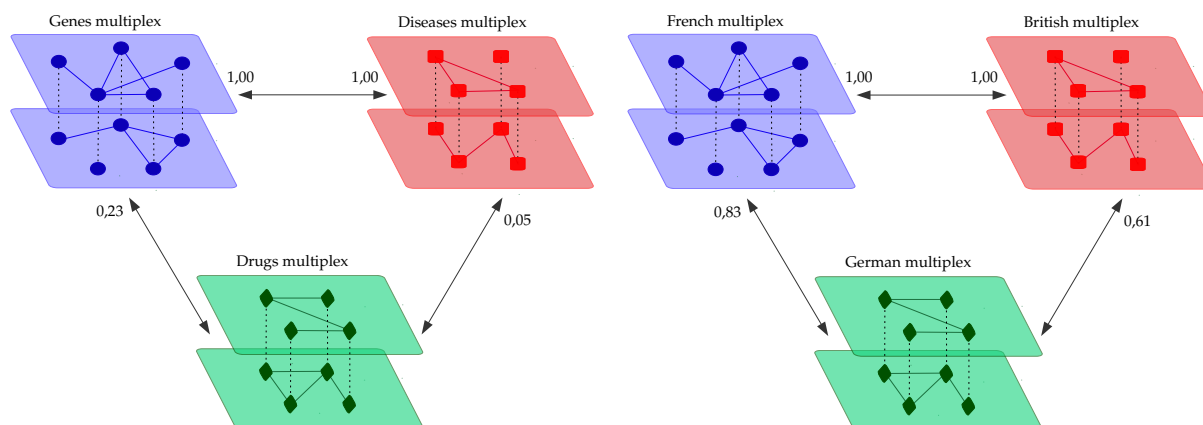

**Fig. S10.** Illustration of the overlaps between the different bipartite networks. We take all the nodes of gene multiplex network (French multiplex network) and all the nodes of the disease monoplex network (British multiplex network) present in the bipartite network between both multiplex networks. For the LOOCV we take only diseases (British airports) associated with at least two genes (French airports). The values in each arrow correspond to the overlaps. For the biological networks, the overlap between the genes and diseases present in the gene-disease bipartite network is equal to 1.00 (all the nodes extract from the gene-disease bipartite network are in this bipartite network). The overlap between the genes present in the gene-disease bipartite network and genes presents the gene-drug bipartite network is equal to 0.23. The overlap between the diseases present in the gene-disease bipartite network and the diseases present in the disease-drug bipartite network is equal to 0.05. Same interpretation should be given for the airports networks.

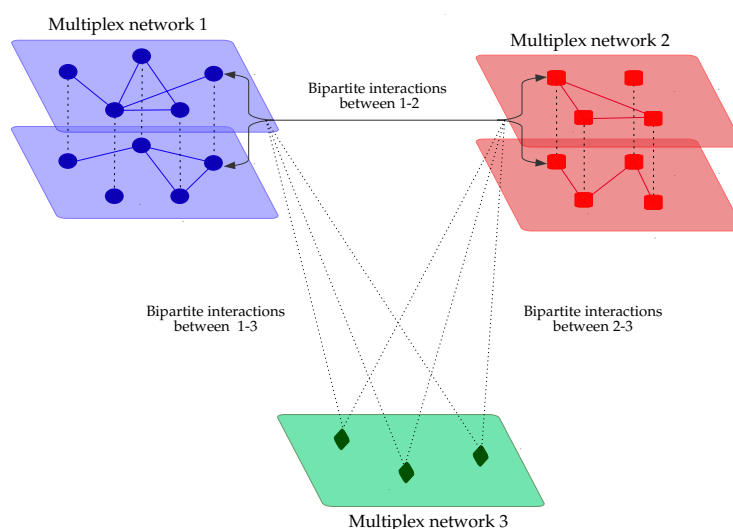

**Fig. S11.** Strategy used to increase the connectivity of the gene-drug and disease-drug bipartite networks. We added simulated drug nodes as transit nodes (green nodes in green layer) linking diseases to genes. For each association between the multiplex network 1 (blue) and multiplex network 2 (red), we simulate the addition of 1, 2, 3, 5 and 10 transit nodes (here three transit nodes are represented for one association).

bipartite networks. It is expected if the bipartite networks that were highly connected for the multilayer networks are replaced by random ones, we reduce the predictive power, until observing the same results as obtained with only two multiplex networks.

Step by step, we replace some parts of the bipartite networks with shuffled (random) networks, first with 10% of random links, then 20%, then 50%, and finally 100%, and the observation is very clear more the bipartite networks are perturbed more the predictive power decrease. At the end with fully shuffled bipartite networks, we observed a result similar to the one obtained with only two multiplex networks. The detailed of the results are given for the airports multilayer network in Fig. S12.A and Fig S13.A and for the biological multilayer network in the Fig. S12.B and Fig. S13.B.

The method is a good way to test if the adding of a new network contributed to the whole network. In other words, we have a method to test the Signal-to-noise ratio.

## B. Exploration of parameter space.

Our analysis focus on two different multilayer networks. A small airports multilayer network composed of three multiplex networks which represents: a French airports multiplex network, a British airports multiplex network, and a German airports multiplex network. In each multiplex network, the nodes represent airports, and the edges the national flight connections between these airports. All these multiplex networks are linked with bipartite networks that correspond to transnational flight (for details see section 3.A). The second network is a large biological multilayer network composed of: a gene multiplex network, a disease monoplex network, and a drug multiplex network. Each multiplex network is connected to the others thanks to bipartite networks association (for details see section 3.B).

### First step: Definition of the sets of parameters for MultiXrank

The choice of the sets of input parameters are delicate because we need to take a step size small enough to explore all the space but not so much to avoid a drastic increase in the running time.

Some parameters do not need to be changed across the exploration, the global restart ( $r$ ) does not affect the solution whatever the other parameters as seen in (see section 1.A.1). The probability to restart in a specific multiplex network ( $\eta$ ) only depends on seeds that do not change across the process, so it can be imposed. We also choose to impose the probability to restart in specific layers ( $\tau$ ). Moreover, the diagonal elements of the matrix of the probability of jumping from one multiplex network to another ( $\lambda$ ) are imposed by the anti-diagonal elements of the same row.

So, we decide to test the anti-diagonal  $\lambda$  parameters and the parameters that control the probability to jump from one layer to another in a specific multiplex network ( $\delta$ ).

Then, we run MultiXrank on each set of parameters, that gives output scores for every node in each multiplex network.

### Second step: Construction of the Similarity matrix

To define the similarity between output scores of two different sets of parameters, we have access to two pieces of information: the ranking of the node and its associated value. In other words, we have the ranking distribution and the standard distribution. We tried to combine the Kullback-Leibler measure to a measure about the ranking of the nodes. However, the Kullback-Leibler divergence drives the similarity measure from a distribution form point of view. That seems to be less efficient for the determination of the cluster at the fourth step than only used the ranking distribution. So we adopt the simplest form for the similarity measure, based on a weighted ranking score:

Let define two sets of parameters:  $\alpha, \beta$

$N$  is the number of multiplex network

$m_i$  is the number of nodes associated to the multiplex network  $i$

$r_\alpha^i$  resp.  $r_\beta^i$  is the scores associated to the sets of parameters  $\alpha$  resp.  $\beta$  for the multiplex network  $i$ .

$r_{\alpha\beta}^i$  resp.  $r_{\beta\alpha}^i$  is the distribution of position of the nodes associated to the sets of parameters  $\alpha$  resp.  $\beta$  for the distribution associated to  $\beta$  resp.  $\alpha$ , for the multiplex network  $i$ .

$$S_{\alpha\beta}^i = \sum_{j=1}^{m_i} \frac{\sqrt{[(r_\alpha^i)_j - (r_{\beta\alpha}^i)_j]^2 + [(r_\beta^i)_j - (r_{\alpha\beta}^i)_j]^2}}{(\frac{r_\alpha^i + r_\beta^i}{2})^2} \quad [31]$$

$$S_{\alpha\beta} = \sqrt{\sum_{i=1}^N \frac{(S_{\alpha\beta}^i)^2}{m_i}} \quad [32]$$

### Third step: Projection of the Similarity matrix into the PCA space

We need to represent each similarity vector that is an M-dimensional representation (where M is the number of sets of parameters) into a unified and two-dimensional space. To make it, we use the PCA that is a suitable way to represent in low dimension the spreading of the data, by variance optimization.

### Fourth step: Clustering the PCA space into sub-regions of stability

After representing the data in a two-dimension space we need to cluster it, to do so, we apply the k-means clustering algorithm on the nodes represented in the PCA space. The nodes gathered in a specific cluster correspond to similar output scores resulting from sets of parameters.

The number of clusters chosen is an important parameter that has to be tuned, depending on the dispersion of the data in the PCA space. Moreover, the choice of the clustering method can be discussed: we do not see any remarkable difference between k-means, spectral clustering, and agglomerative clustering, so we adopt the simplest one. However, it is to note that the clustering is sensitive to the chosen metric, for instance for agglomerative clustering the Manhattan

metric offers better results than euclidean, L1 or cosine metrics.

**Fifth step:** *Checking the stability the top ranking nodes in each cluster*

After clustering each output score on the PCA space, we need to evaluate if the output scores that are aggregated in the same cluster share a common ranking, whatever the multiplex network. To determine it, we display the top-K nodes (with K equal to 1, 3, 5, 10, 20, 100) network nodes of each cluster and we check if these nodes are common in the solution of all the set of parameters (represent as nodes in the PCA space). The ideal case is that all the network nodes are common in all the distribution of a specific cluster.

A particular difficulty with multilayer comes from the different contributions of multiplex networks, some multiplex networks may have an easy PCA representation and cluster very well every node, but some others can be "messy". This behavior is illustrated by the first multiplex network in Fig. S14, which has many more than ten nodes in the set of the top-10 nodes for multiplex network 1, whereas, in multiplex networks 2 and 3, we see that there are only ten nodes in the top-10.

The projection into the PCA space of the output scores of the sets of parameters shows different behavior depending on the network. For instance, in Fig. S14 we show that the two first components only gather 62.1% of the total variance, and we observe a continuous aspect of the data that traduce a wide variety of results propose by the random walk and a non-unique solution under the variety of input parameters. In this case, the parameters affect drastically the output scores. A trick to fix this issue is to use the consensus ranking that results from averaging all the ranking gave by each set of parameters to extract an average behavior. Fig. S14.B-D can be used to this end. For instance, the top-3 in the first multiplex network is the nodes: 7, 169, and 199, for the second multiplex network: 17, 28, and 53, for the third multiplex network: 38, 7 and 166.

Very different behavior is observed in Fig. S15 where the two firsts components gathered 97.6% of the total variance. The cluster are well separated and inside we observe a proper behavior, moreover, the top-ranking nodes are very common between each set of parameters.

This reflects two very different kinds of networks, on the one hand, scattered behavior network with high impact on the input parameters, on the other hand, stable behavior network with well-established sub-regions and robustness under the change of input parameters in each separated cluster.

The spreading of data observed in Fig. S14 can be also observed about the clustering in the PCA space of the data associated with the multiplex network 1 (Fig. S16.F). In this figure, we observe a continuous projection of the data along the y axis. Moreover, this behavior is reflected in two other figures: in Fig. S16.B, where we observe a large number of top-100 nodes (several blue pics), and in Fig. S16.D where we see an enhanced difficulty of well clustering the nodes in the PCA space. The previous observation is not found for the data associated with the multiplex network 2, where the PCA unambiguously divides the space.

Finally, we see that in the PCA space associated with multiplex network 2 only 4 clusters are enough to separate correctly the whole space. Whereas, for the multiplex network 1, we need to use at least 8 clusters. Thus in the total space created with the formula [30], we also need to use more than 4 clusters to properly divided the space. In conclusion, the heterogeneity of the total space is driven by the first multiplex network (gene multiplex network) and find in the total network, but the ability to cluster is still possible thanks to a robust second network (disease monoplex network).

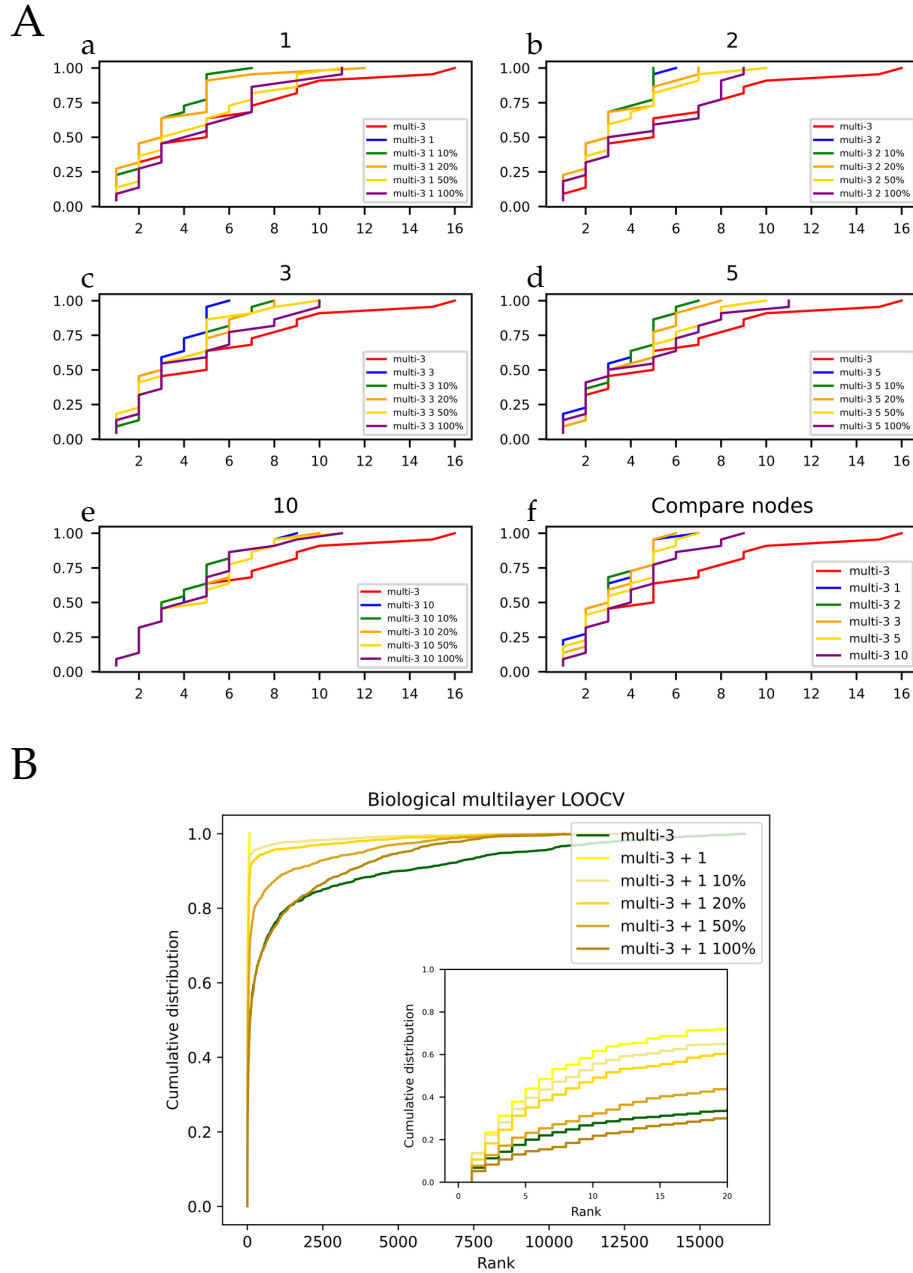

**Fig. S12.** Cumulative Distribution Functions (CDFs) representing the ranks of the left-out nodes for the perturbation protocol of the high connectivity case for LOOCV. A: Representing the CDFs of the left-out nodes for the airports multilayer network for 5 case studies of high connectivity cases: the case where we add 1, 2, 3, 5, or 10 transit nodes in the German airports (edges in the French-German and British-German airports bipartite networks) multiplex network to artificially increase the connectivity of the nodes of the bipartite networks between the French airports multiplex network and the British airports multiplex network (Fig.A.a-e). In each figure, we display the CDF associated with the multilayer networks composed of the three multiplex networks: French, British, and German multiplex networks (multi3), the CDF associated with the high connectivity case, and the CDFs resulting from the perturbation of the French-German airports bipartite network and the British-German airports multiplex network designed to artificially increase the connectivity (by adding transit nodes). We randomized, 10%, 20%, 50%, and 100% of these bipartite networks. Fig. A.f represents the distribution for the 3-multiplex network associated with the 5 high connectivity cases described previously compare to the 3-multiplex network without transit nodes. B: Representing the CDFs of the left-out nodes for the biological multilayer network composed of the gene, drug multiplex networks, and the disease monoplex network: without transit node (multi3), with one transit node (which artificially increased the connectivity) in the gene-drug bipartite network and the disease-drug bipartite network for each gene-disease associations (multi3+1), the previous system with 10% of randomized edges in the gene-drug bipartite network and the disease-drug bipartite network (multi+1 10%), the previous system with 20% in these bipartite networks (multi+1 20%), the previous system with 50% in these bipartite networks (multi+1 50%), the previous system with 100% in these bipartite networks (multi+1 100%).

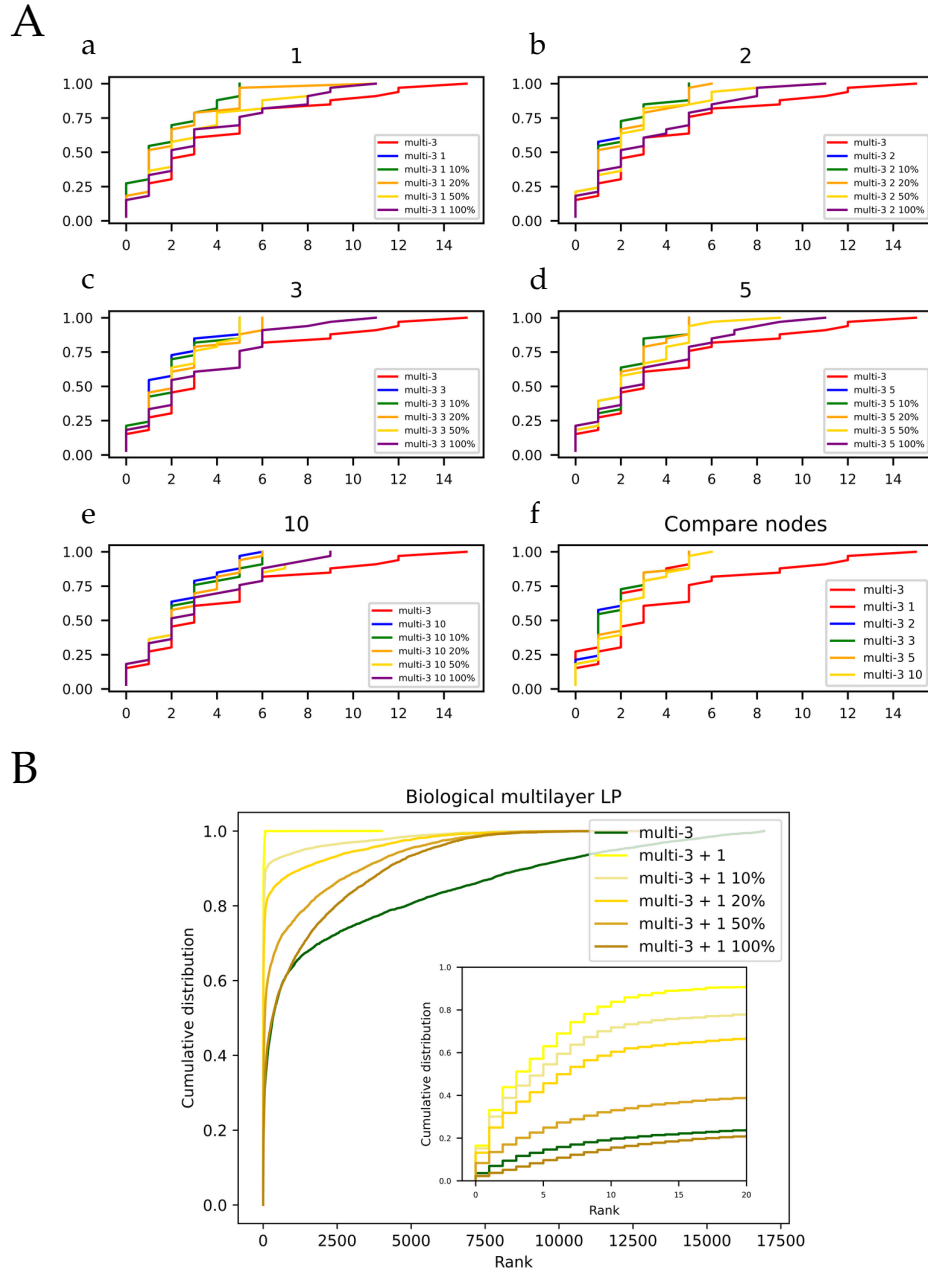

**Fig. S13.** Cumulative Distribution Functions (CDFs) representing the ranks of the left-out nodes for the perturbation protocol of the high connectivity case for LP. A: Representing the CDFs of the left-out nodes for the airports multilayer network for 5 case studies of high connectivity cases: the case where we add 1, 2, 3, 5, or 10 transit nodes in the German airports (edges in the French-German and British-German airports bipartite networks) multiplex network to artificially increase the connectivity of the nodes of the bipartite networks between the French airports multiplex network and the British airports multiplex network (Fig.A.a-e). In each figure, we display the CDF associated with the multilayer networks composed of the three multiplex networks: French, British, and German multiplex networks (multi3), the CDF associated with the high connectivity case, and the CDFs resulting from the perturbation of the French-German airports bipartite network and the British-German airports multiplex network designed to artificially increased the connectivity (by adding transit nodes). We randomized, 10%, 20%, 50%, and 100% of the edges of these bipartite networks. Fig. A.f represents the distribution for the 3-multiplex network associated with the 5 high connectivity cases described previously compare to the 3-multiplex network without transit nodes. B: Representing the CDFs of the left-out nodes for the biological multilayer network composed of the gene, drug multiplex networks, and the disease monoplex network: without transit node (multi3), with one transit node (which artificially increased the connectivity) in the gene-drug bipartite network and the disease-drug bipartite network for each gene-disease associations (multi3+1), the previous system with 10% of randomized edges in the gene-drug bipartite network and the disease-drug bipartite network (multi+1 10%), the previous system with 20% in these bipartite networks (multi+1 20%), the previous system with 50% in these bipartite networks (multi+1 50%), the previous system with 100% in these bipartite networks (multi+1 100%).

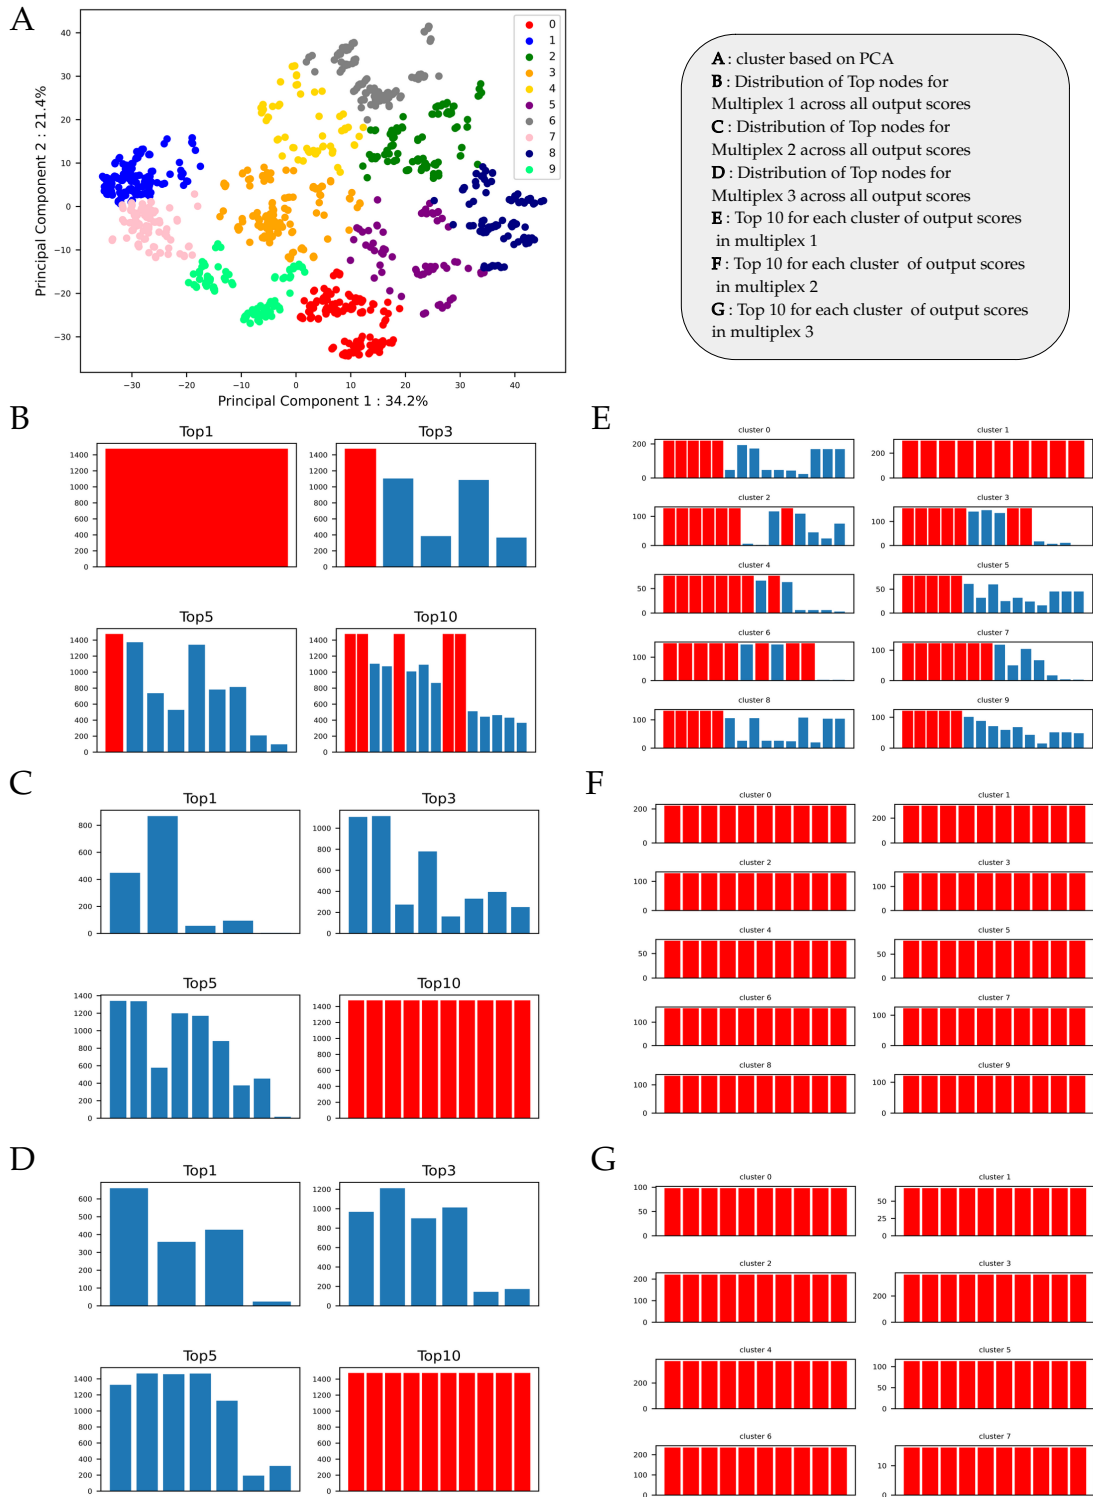

**Fig. S14.** A: Clustering in the PCA space of the output scores obtained with MultiXrank on the airports multilayer network composed of the French, British, and German airports multiplex networks described in section 3.A, using different sets of parameters. B-D: Comparisons of the top-1, top-3, top-5, and top-10 nodes obtained for the French airports multiplex network (B), for the British airports multiplex network (C), and for the German airports multiplex network (D), for the different sets of parameters. E-G: Top-10 nodes for each cluster defined from the PCA space (A), for the French airports multiplex network (E), for the British airports multiplex network (F), and for the German airports multiplex network (G). The bar is colored in red when a node is found in all top-K scores (K is equal to 1, 3, 5, and 10), and in blue otherwise.

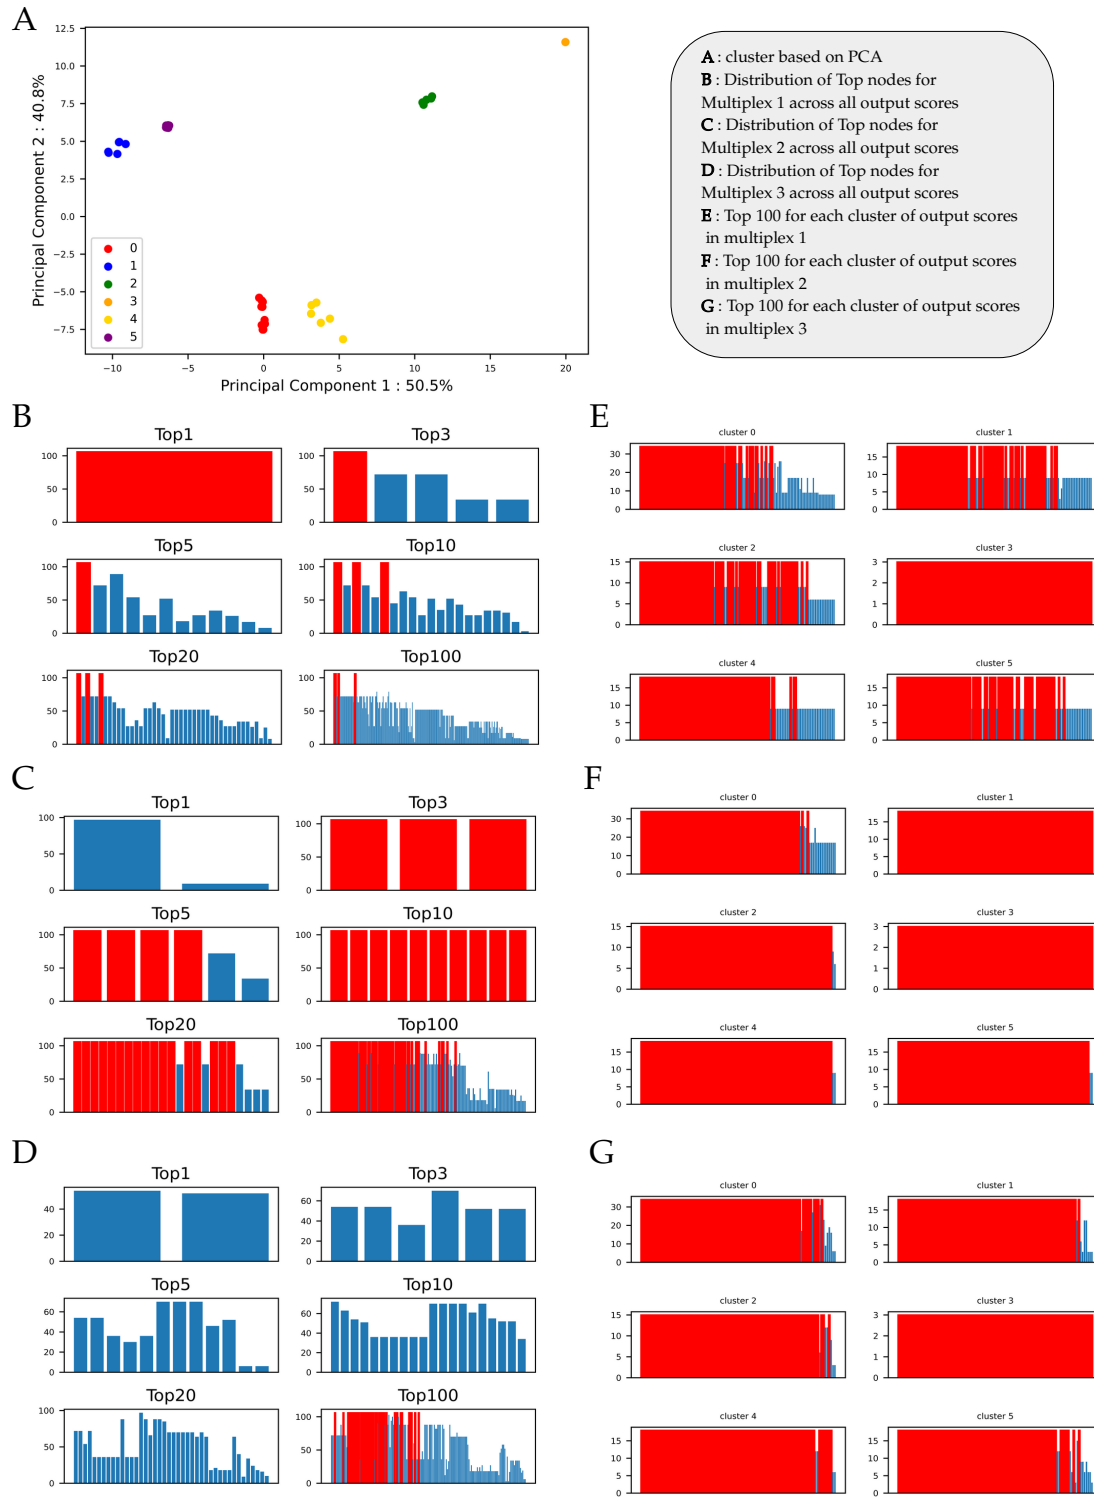

**Fig. S15.** A: Clustering in the PCA space of the output scores obtained with MultiXrank on biological multilayer composed of genes, drug multiplex networks, and a disease monoplex network as described in section 3.B, using different sets of parameters. B-D: Comparisons of the top-1, top-3, top-5, top-10, top-20 and top-100 nodes obtained for the gene multiplex network (B), for the disease monoplex network (C), and for the drug multiplex network (D), for the different sets of parameters. E-G: Top-100 nodes for each cluster defined from the PCA space (A), for the gene multiplex network (E), for the disease monoplex network (F), and for the drug multiplex network (G). The bar is colored in red when a node is found in all top-K scores (K is equal to 1, 3, 5, 10, 20, and 100), and in blue otherwise.

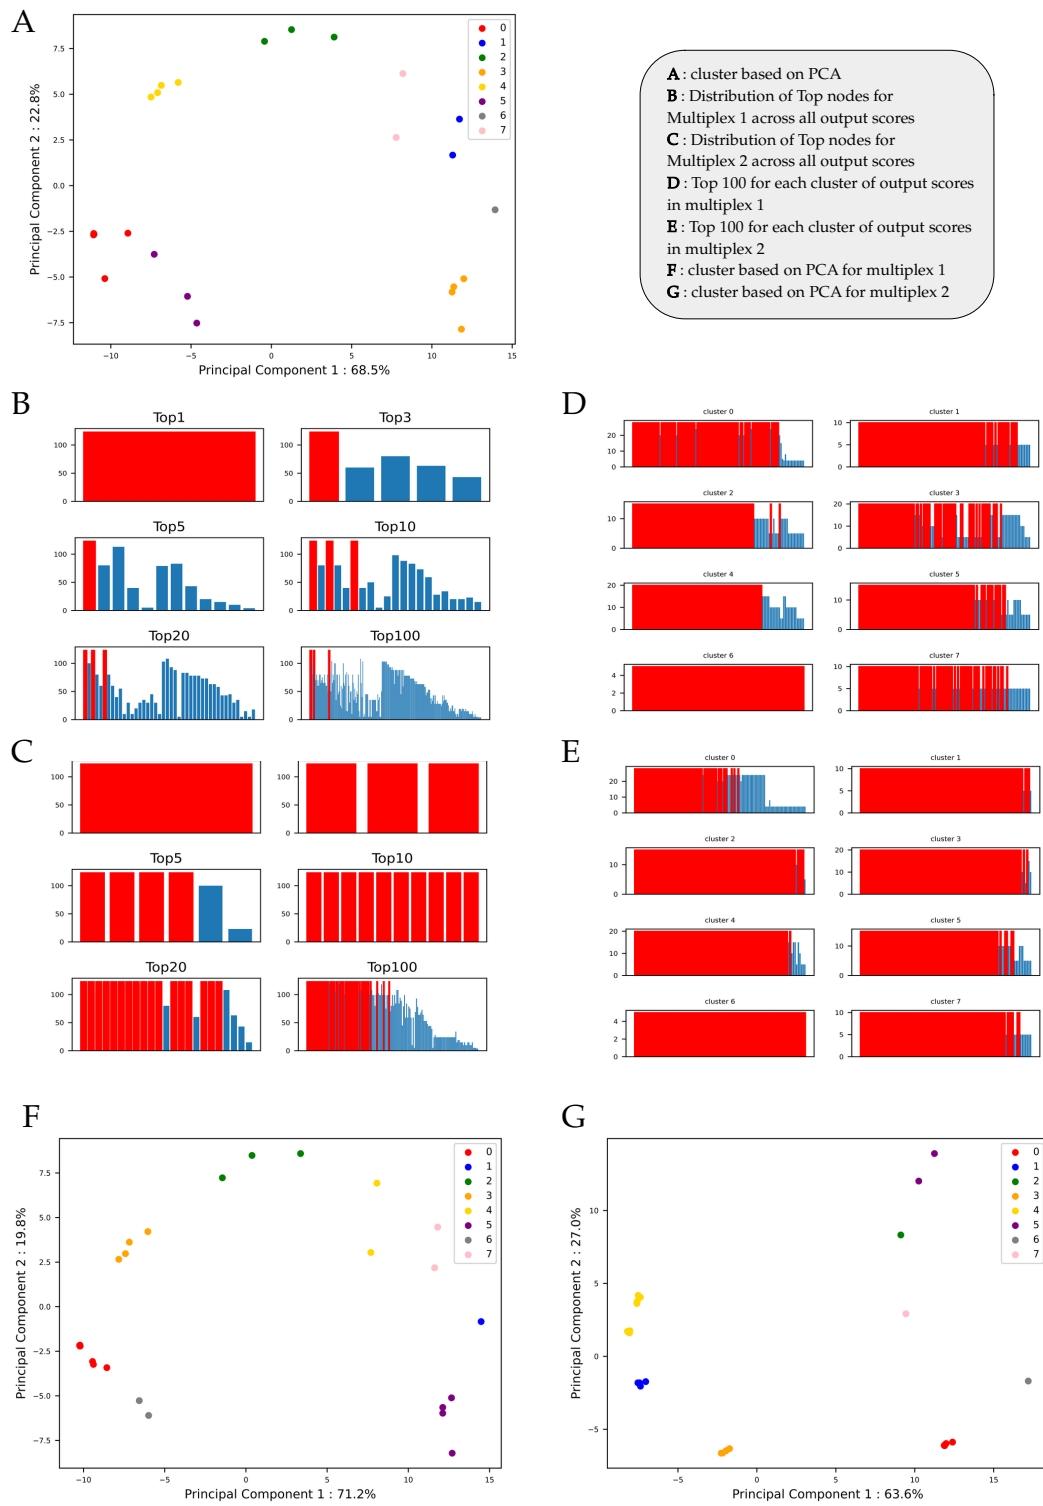

**Fig. S16.** A: Clustering in the PCA space of the output scores obtained with MultiXrank on biological multilayer composed of gene multiplex network, and a disease monoplex network as described in section 3.B, using different sets of parameters. B-C: Comparisons of the top-1, top-3, top-5, top-10, top-20 and top-100 nodes obtained for the gene multiplex network (B), for the disease monoplex network (C), for the different sets of parameters. D-E: Top-100 nodes for each cluster defined from the PCA space (A), for the gene multiplex network (D), for the disease monoplex network (E). The bar is colored in red when a node is found in all top-K scores (K is equal to 1, 3, 5, 10, 20, and 100) and in blue otherwise. F-G: Clustering in the PCA space of the output scores obtained with MultiXrank on previous biological multilayer when we only consider the genes output scores (F) or only the diseases output scores (G).

## 5. MultiXrank applications:

### A. Node Prioritization in Leukemia.

We take the genes and the drug multiplex networks described in Table S5. We focus on the study of Leukemia, which is a well-studied disease. We choose as seeds one gene and one drug: **HRAS**, which known to be involved in Acute Myeloid Leukemia (AML) (15), and Tipifarnib (**DB04960**), a drug that is being studied in the treatment of AML and other types of cancer (16–18).

We checked the top-10 scoring genes and drugs (Table S6) obtained from MultiXrank, and compared to the literature and the DrugBank database information, to determine if predictions are relevant regarding to the current knowledge.

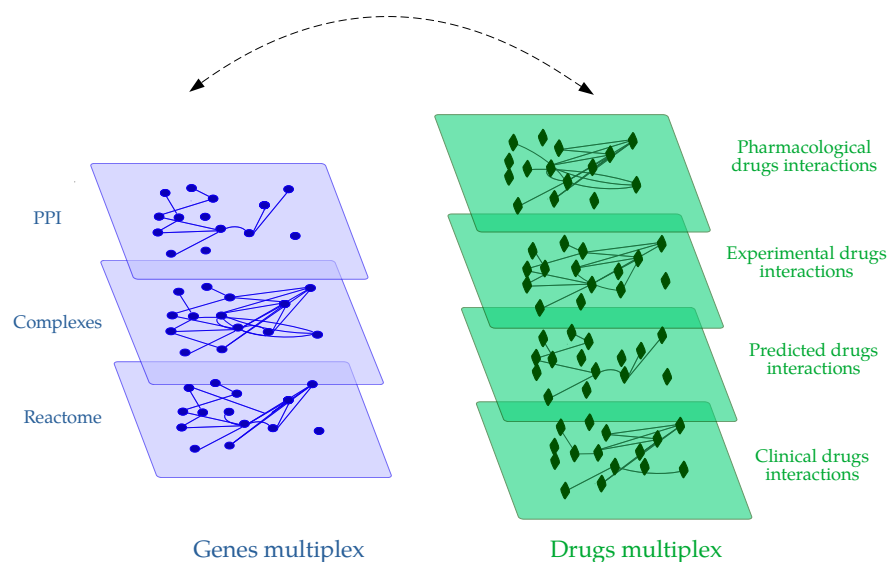

**Fig. S17.** Multilayer network composed of a genes and drug multiplex networks and its associated bipartite network (represented as bipartite interactions).

Top-10 genes (at least one reference was found in the literature for each gene):

1. CYP3A4 is known to be implicated in Leukemia [<https://doi.org/10.1073/pnas.95.22.13176>].
2. FNTB is the target of Tipifarnib (our seed drug) according to DrugBank.
3. RAF1 is a well-known Leukemia-associated gene [ORPHA → RAF1 - Raf-1 proto-oncogene, serine/threonine kinase].
4. RASGRP1 has been linked with Leukemia previously [<https://doi.org/10.1038/leu.2011.328>].
5. DGKZ knockdown can induce apoptosis in human AML HL-60 cells through the MAPK/survivin/caspase pathway [<https://doi.org/10.1691/ph.2019.9386>].
6. RIN1 plays a role in the maintenance of the abnormal RTK signaling in Chronic Myeloid Leukemia [<https://doi.org/10.1007/s13277-015-3772-9>].
7. BRAF mutations were identified in AML patients with monocytic differentiation [<https://doi.org/10.1080/10428194.2016.1213830>].
8. RASA1 is involved in several cancer types, including Leukemia [<https://doi.org/10.3892/or.2020.7807>].
9. ARAF: A study [<https://doi.org/10.1111/j.1600-0463.2005.apm1130108.x>] found ARAF gene mutation in MOLT-4 Leukemia cell line.
10. AURKA: A significant association between over-expression of AURKA and cytogenetic abnormalities was found in AML patients [<https://doi.org/10.1016/j.leukres.2010.07.034>].

Top-10 drugs (we first parsed DrugBank to identify the indications for each drug and further surveyed the literature to find additional information):

| $r$ | $\delta$                                  | $\tau$                                                                       | $\lambda$                                              | $\eta$                                    | $K$ |
|-----|-------------------------------------------|------------------------------------------------------------------------------|--------------------------------------------------------|-------------------------------------------|-----|
| 0.7 | $\begin{bmatrix} 1/2 & 1/2 \end{bmatrix}$ | $\begin{bmatrix} 1/3 & 1/3 & 1/3 & 0 \\ 1/4 & 1/4 & 1/4 & 1/4 \end{bmatrix}$ | $\begin{bmatrix} 1/2 & 1/2 \\ 1/2 & 1/2 \end{bmatrix}$ | $\begin{bmatrix} 1/2 & 1/2 \end{bmatrix}$ | 10  |

| multiplex network | Layer                              | Nodes | # interactions |
|-------------------|------------------------------------|-------|----------------|
| 1                 | PPI                                | genes | 143 652        |
| 1                 | Complexes                          | genes | 63 561         |
| 1                 | Reactome                           | genes | 194 500        |
| 2                 | clinical drugs interactions        | drugs | 14 909         |
| 2                 | experimental drugs interactions    | drugs | 843            |
| 2                 | predicted drugs interactions       | drugs | 2 080          |
| 2                 | Pharmacological drugs interactions | drugs | 48 514         |

| multiplex network | # Nodes |
|-------------------|---------|
| 1                 | 16 967  |
| 2                 | 1559    |

| Bipartite networks | # interactions |
|--------------------|----------------|
| 2-1                | 30 895         |

**Table S5.** Networks specificities and parameters for the genes and drug multiplex networks.

| genes   | scores   | drugs   | scores   |
|---------|----------|---------|----------|
| CYP3A4  | 0.009444 | DB00637 | 0.000357 |
| FNTB    | 0.009263 | DB01380 | 0.000350 |
| RAF1    | 0.001001 | DB00630 | 0.000326 |
| RASGRP1 | 0.000982 | DB00398 | 0.000313 |
| DGKZ    | 0.000780 | DB00399 | 0.000252 |
| RIN1    | 0.000745 | DB00773 | 0.000248 |
| BRAF    | 0.000225 | DB01254 | 0.000184 |
| RASA1   | 0.000204 | DB01268 | 0.000165 |
| ARAF    | 0.000196 | DB06589 | 0.000114 |
| AURKA   | 0.000195 | DB00530 | 0.000096 |

**Table S6.** MultiXrank scores for multilayer network composed of a genes and drug multiplex networks

1. DB00637 (Astemizole) belongs to a drug class that was validated for its activities against human primary AML samples [<https://doi.org/10.1038/s41408-018-0087-2>].
2. DB01380 (Cortisone acetate): This drug has two targets, ANXA1 and NR3C1, which are part of the top-10 predicted genes. Moreover, cortisone acetate was shown to dramatically reduce the size of lymphoid tumors or Leukemia [[doi:10.1172/JCI102317](https://doi.org/10.1172/JCI102317)].
3. DB00630 (Alendronate): Some preliminary experiments show a benefit for the treatment of osteopenia/osteoporosis with Alendronate in children with Acute Lymphoblastic Leukemia [<https://doi.org/10.1097/mpb.0b013e318142b7a1>].
4. DB00398 (Sorafenib) is a drug used for the treatment of advanced renal cell carcinoma, and some studies mention its impact on Leukemia [<https://doi.org/10.1038/sj.leu.2404508>].
5. DB00399 (Zoledronic acid) is a drug used to prevent skeletal fractures in patients with cancers such as multiple myeloma and prostate cancer, and some studies show interesting links with Leukemia [<https://doi.org/10.3892/mmr.2016.5957>].
6. DB00773 (Etoposide) is used for first-line treatment in patients with small-cell lung cancer. It is also used to treat other malignancies such as Lymphoma, Nonlymphocytic Leukemia (source:DrugBank).
7. DB01254 (Dasatinib) is used in patients with Chronic Myelogenous Leukemia (source:DrugBank).
8. DB01268 (Sunitinib): A phase I/II study of sunitinib and intensive chemotherapy for AML patients with FLT3 mutations has been achieved achieved with encouraging results [<https://doi.org/10.1111/bjh.13353>].
9. DB06589 (Pazopanib): This drug is in clinical trial phase II for patients with AML [<https://doi.org/10.1007/s00277-019-03651-9>].
10. DB00530 (Erlotinib) is an inhibitor of the epidermal growth factor receptor (EGFR) tyrosine kinase that is used in the treatment of several types of cancer, and some references exist for Leukemia [<https://doi.org/10.4161/cc.22382>].

In conclusion, all the top-ranked genes and drug prioritized with the HRAS and Tipifarnib seeds have links with Leukemia. These results illustrate the efficiency of MultiXrank in a prioritization task.

## **B. Node Prioritization to identify drugs involved in epilepsy and comparison with the Hetionet framework.**

Based on networks described in section 3.C we try to find similar results observed in D.S.Himmelstein et al. (13) for the epilepsy case study. In this study, the authors use a homemade machine learning code based on regularized

logistic regression to predict candidate drugs that can have effects on epilepsy. The algorithm runs on heterogeneous networks and gives back the top-100 most relevant drugs associated with epilepsy. Then these drugs are classified into three classes: anti-ictogenic (AIGD) that have seizure suppressing effect (77 drugs), unknown (UNKD) that have no established effect on the seizure threshold (8 drugs), or ictogenic (IGD) with seizure generating effect (15 drugs).

The first step consists in importing the heterogeneous networks from Hetionet and convert them into a universal multilayer network and on a suitable edgelist format (Fig S6) for MultiXrank. Then we run our framework to predict output scores of drugs for the multilayer networks with epilepsy node (OID:1826) considered as the seed node. Then we check for different sets of parameters (Fig S18) if we identify the same top-100 set of drugs as the one predicted in D.S.Himmelstein et al. (13).

The analysis of Fig. S18 shows that almost all predicted drugs (99%) are found in the top-500 by our MultiXrank and 59% of drugs are in the top-100 and 80% in the top-200. Moreover, we can see that the tuning of the input parameters increases the number of candidate drugs found in the top-100 from 54 for the set of parameters number 2 to 59 for the set of parameters number 4. It is important to note that the only parameter that has been changed is the lambda matrix that corresponds to the probability of jumping from one multiplex network to another.

Finally, we check the 41% other drugs that are found by MultiXrank with the set of parameters 4, in the top-100 of candidate drugs for epilepsy. Table S7 displays all the classes of drugs that are associated with at least seven drugs. We will determine to what extent these other drugs are relevant for the epilepsy case study. We will focus on three classes of drugs extracted from Table S7: Cytochrome P-450 Substrates, Analgesics, and Indoles. We remind that some drugs have several classifications, for instance: Among the 27 different drugs overall in the three classes. 24 are Cytochrome P-450 Substrates, 17 are Analgesics (14 are both Cytochrome P-450 Substrates and Analgesics), 8 are Indoles (5 are both Cytochrome P-450 Substrates and Indoles), and all the Indoles drugs are also Analgesics.

A recent study has shown in mice, that spontaneous recurrent seizures modify Cytochrome P-450 expression in the liver and the hippocampus. The authors conclude with the hypothesis that nuclear receptors or inflammatory pathways can be considered as candidate mechanisms of Cytochrome P-450 regulation during seizures (19). A recent review indicates preclinical evidence that tends to show that anti-epileptic drugs can be used as Analgesics in patients with inflammatory pain, and can contribute to the improvement of the treatment of various inflammatory pain states (20). Lately, another study on rats, evaluate the anti-epileptic effect of new Indole derivatives. This study exhibits that some Indole derivatives induced a decreasing susceptibility to seizures (21).

To conclude this brief review reinforces MultiXrank as an efficient method for node prioritization.

## C. Supervised classification of gene-disease associations.

To determine if MultiXrank is suitable for the prediction of new gene-disease associations, we designed a protocol that consists in using MultiXrank output scores from an old version of a gene-disease dataset (DisGeNET v2.0, 2014) to train a binary classifier (random forest), and then to test if this classifier can predict associations that are found in an updated version of the same dataset (DisGeNET v7.0, 2020).

### C.1. Supervised classification protocol.

It is important to note that the process is the same for multilayer networks composed of two or three multiplex networks. So here we specified the process for the two multiplex networks case.

#### First step: Creation of the training dataset

The training dataset is created based on the 2014 gene-disease associations of DisGeNET database (v2.0), each association is associated with a score depending on the number of sources that report the association. We choose a threshold equal to 0.5, in this case, we obtain 1980 associations, that constitute our positive dataset (label equal to 1) On the other hand, we generate a negative set of 1980 associations (label equal to 0) defined as a subset of the following one:  $\{(i, j) \in (\text{Gene node}, \text{Disease nodes}) \setminus \{(i, j) \in \text{Disgnet v2.0}\}\}$ .

Finally, the training dataset is composed of the merging of the two previous datasets.

#### Second step: Running MultiXrank for all associations

Then for all associations defined in the training dataset, we run MultiXrank on the multilayer network composed of two multiplex networks, one composed of three layers of genes (gene multiplex network) and a second composed of a diseases similarity network (disease monoplex network), see section 3.B for more details on the networks. The bipartite network is composed of the full gene-disease association defined by DisGeNET v2.0. The parameters chose for the MultiXrank are defined in Table S8.

For each pair defined by the training dataset, we used both nodes as seeds nodes, and we save the scores defined by the MultiXrank for each multiplex network. Then these scores are merge and convert into a sparse matrix. Finally, we

Distribution of drugs : parameter 1

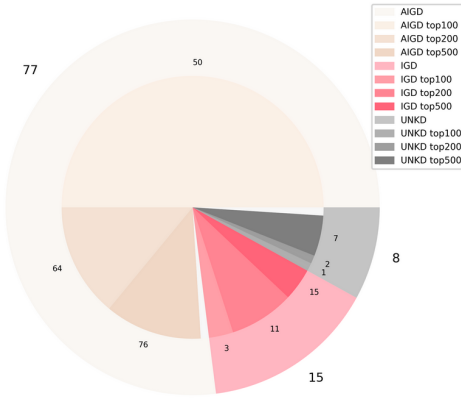

Distribution of drugs : parameter 2

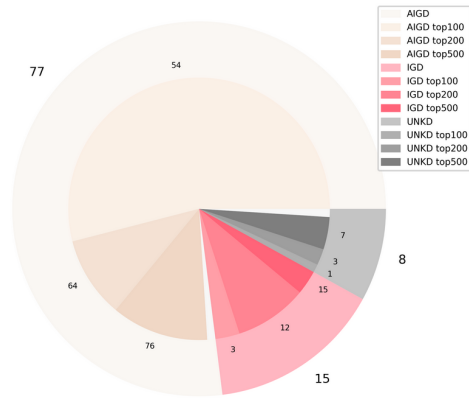

Distribution of drugs : parameter 3

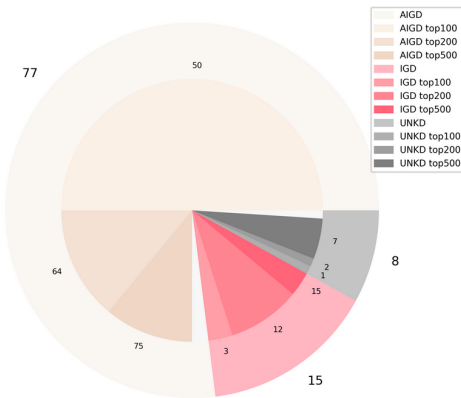

Distribution of drugs : parameter 4

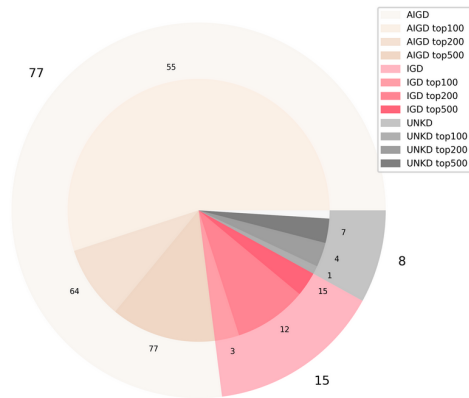

**Fig. S18.** Distribution of top-predicted drugs for different sets of parameters of MultiXrank compared with Hetionet predictions, for the epilepsy case study. AIGD represents anti-ictogenic drugs that have a seizure suppressor effect (in beige), IGD represents ictogenic drugs (in pink), and UNKD represents drugs with unknown effects (in grey). For each set of parameters (1, 2, 3 or 4) we display in the outer circle the number of AIGD, IGD, and UNKD drugs found by Hetionet, and in the inner pie chart, the number of the same AIGD, IGD, and UNKD find in the top-100, top-200, and top-500 by MultiXrank. The number of nodes for top-500 includes the nodes found in the top-200, and the top-200 include the nodes found in the top-100. It is to note that the white part of the pie chart correspond to the fraction of the drugs that are out of the top-500 drugs.

split the large sparse matrix into sub-matrices to store and then re-use it, during the training step. This choice is motivated by the RAM saturation issue and the wish to optimize the memory space needed.

### Third step: Training the binary classifier (Random forest)

The scores obtained with MultiXrank are the base of the training step. The scores encode the proximity of all the nodes of both multiplex networks to the seeds nodes that are (un)associated with each gene-disease association. The question posed by the ability to train a classifier thanks to the MultiXrank scores is the same as the question that consists in wonder if the topology of the networks encodes the biology that makes some genes and some diseases associated or not, and if MultiXrank can catch it. The way used to train the classifier from MultiXrank process is inspired by the method in Liu et al. (22). However, we adapt their process to use it, the details of the protocol are explained in Fig S19.

The choice of the binary classifier is a difficult one. Each method has its own drawbacks and advantages, thus in our case, we defined some characteristics that the method needs to gather. It needs to be robust, interpretable, and it must not overfit the training set. The overfitting is a well-known issue in the case of the decision tree, that excludes this method, however, their ability to be easily interpretable is an appealing advantage. So, we choose using random forest as a good compromise between stability, overfitting, and interpretability.

The parameters of the random forest for the two multiplex networks are described in Table S9 (we choose the model

| Drugs class                            | N  | Drugs class                                 | N |
|----------------------------------------|----|---------------------------------------------|---|
| Cytochrome P-450 Substrates            | 24 | Serotonin Modulators                        | 9 |
| Agents that produce hypertension       | 18 | Serotonin Receptor Agonists                 | 9 |
| Central Nervous System Depressants     | 18 | Serotonin 5-HT1 Receptor Agonists           | 9 |
| Neurotransmitter Agents                | 17 | Cytochrome P-450 CYP2D6 Substrates          | 9 |
| Analgesics                             | 17 | Cytochrome P-450 CYP2C9 Substrates          | 8 |
| Heterocyclic Compounds Fused-Ring      | 15 | Indoles                                     | 8 |
| Cytochrome P-450 Enzyme Inhibitors     | 14 | Analgesics Non-Narcotic                     | 8 |
| Cytochrome P-450 CYP3A4 Substrates     | 14 | Agents causing hyperkalemia                 | 8 |
| Amines                                 | 12 | Cytochrome P-450 CYP2C19 Substrates         | 7 |
| Cytochrome P-450 CYP1A2 Substrates     | 12 | Cytochrome P-450 CYP3A4 Inhibitors          | 7 |
| Serotonergic Drugs                     | 11 | Enzyme Inhibitors                           | 7 |
| Antidepressive Agents                  | 10 | Biogenic Amines                             | 7 |
| Serotonin Agents                       | 10 | Biogenic Monoamines                         | 7 |
| Peripheral Nervous System Agents       | 10 | Selective Serotonin 5-HT1 Receptor Agonists | 7 |
| Antimigraine Preparations              | 10 | Selective Serotonin Agonists                | 7 |
| Cardiovascular Agents                  | 10 | Serotonin 1b Receptor Agonists              | 7 |
| Sensory System Agents                  | 10 | Serotonin 1d Receptor Agonists              | 7 |
| P-glycoprotein substrates              | 9  | Triptans                                    | 7 |
| Drugs that are Mainly Renally Excreted | 9  | P-glycoprotein inhibitors                   | 7 |

**Table S7.** Drugs classification of the 41 drugs predicted in the top-100 of MultiXrank with the set of parameters 4 that are not predicted in the top-100 predicted drugs of Hetionet. The first column corresponds to the drug class of drugs and the second to the number of times (N) where this class is found in the 41 drugs predicted only by MultiXrank, we focus on the classes that are associated with 7 or more drugs.

highlighted in orange).

**Fourth step:** *Creation of the test dataset*

The process to define the test dataset is similar to the one described in the first step, we just used in this case for the bipartite network the gene-disease association defined by the newest version of DisGeNET v7.0 (2020) instead of DisGeNET v2.0 (2014). The positive associations are extracted from the DisGeNET v7.0 (threshold equal to 0.5) and the negative associations are defined as a subset of the following set:  $\{(i, j) \in (\text{Gene node}, \text{Disease nodes}) \setminus \{(i, j) \in \text{Disgnet v7.0}\}$

**Fifth step:** *Evaluation of the binary classifier on the test dataset*

Finally, we run MultiXrank for each positive/negative association defined in the test dataset as described in the fourth step. And, we use these output scores to classify the gene-disease association (Fig. S19) from DisGeNET v7.0 (2020) thanks to the random forest binary classifier training on the data obtained with the gene-disease association of DisGeNET v2.0 (2014). At the end, we compare the classification obtained with the random forest to the expected

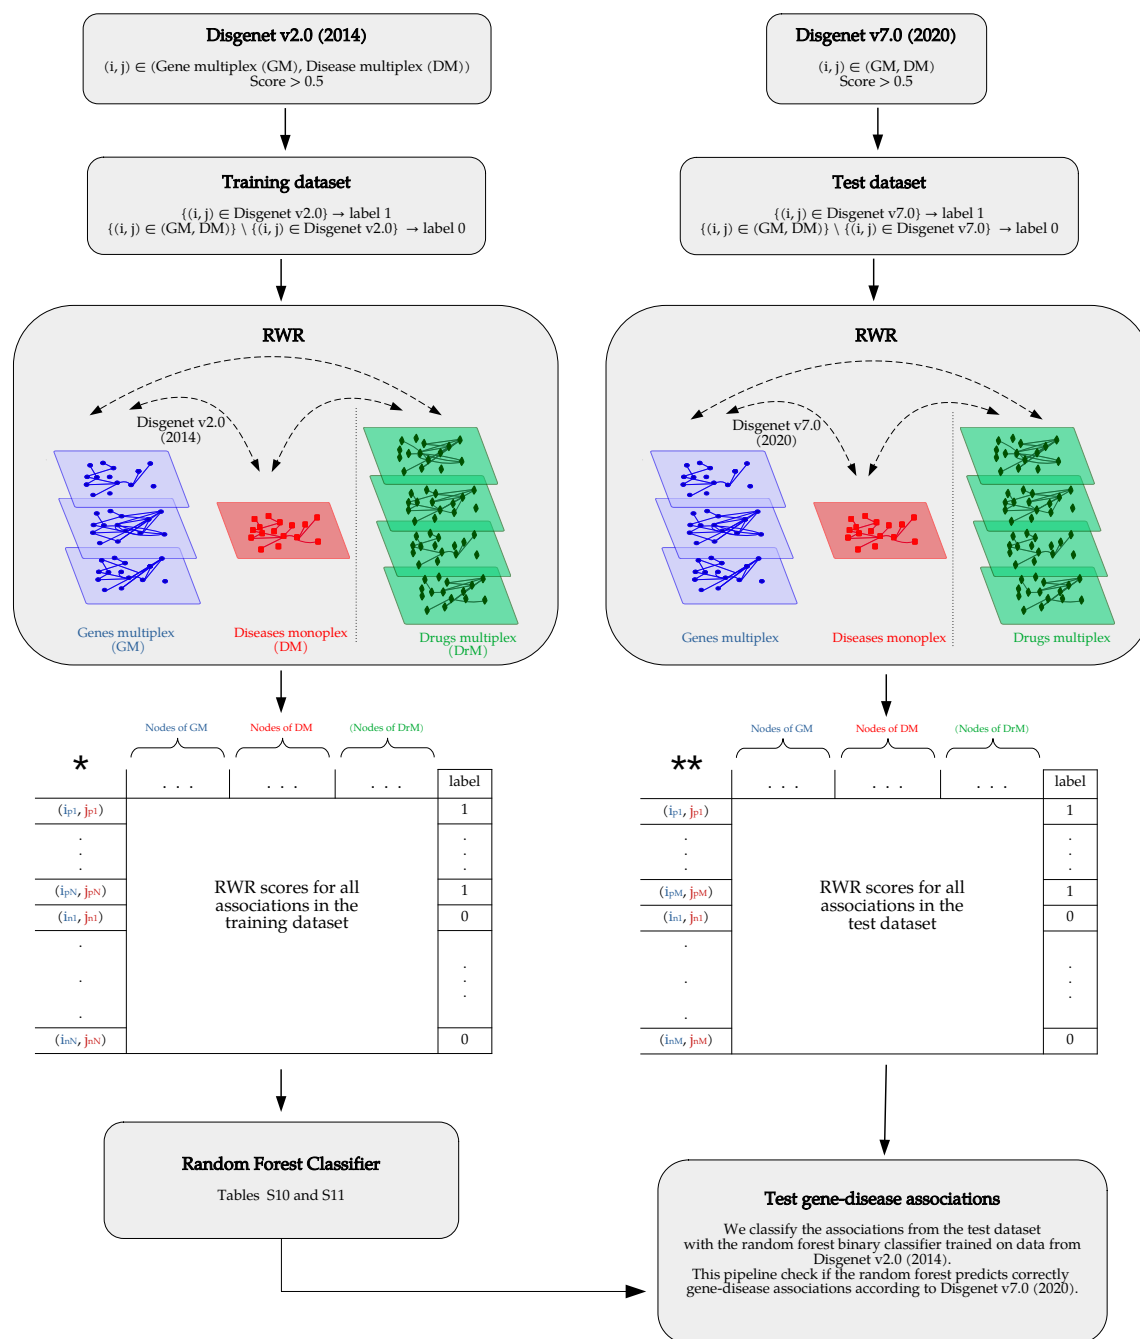

**Fig. S19.** Workflow for the training and the testing of the random forest binary classifier training with MultiXrank output scores. The left workflow represents the training step with the 2014 gene-disease bipartite network (DisGeNET v2.0). After creating both positive (from DisGeNET v2.0) and negative gene-disease associations, we run for each association MultiXrank, and we save the output scores as described in the matrix \*. Then we use this matrix with the label to train a random forest binary classifier. The right workflow represents the test step with the updated (2020) gene-disease bipartite network (DisGeNET v7.0). After creating the positive (from DisGeNET v7.0) and negative gene-disease associations, we run MultiXrank, and we save the output scores as described in the matrix \*\*. The last step consists of using this matrix as an input of the previous trained random forest classifier to predict the labels. Finally, we compare the predictions of the labels by the random forest classifier and the known labels (Tables S9 and S10). The workflow is the same for two or three multiplex networks.

results (associations in/out of DisGeNET v7.0).

| $r$ | $\delta$                                | $\tau$                                                       | $\lambda$                                              | $\eta$                                    | $K$   |
|-----|-----------------------------------------|--------------------------------------------------------------|--------------------------------------------------------|-------------------------------------------|-------|
| 0.7 | $\begin{bmatrix} 1/2 & 0 \end{bmatrix}$ | $\begin{bmatrix} 1/3 & 1/3 & 1/3 \\ 1 & 0 & 0 \end{bmatrix}$ | $\begin{bmatrix} 1/2 & 1/2 \\ 1/2 & 1/2 \end{bmatrix}$ | $\begin{bmatrix} 1/2 & 1/2 \end{bmatrix}$ | 'all' |

| $r$ | $\delta$                                      | $\tau$                                                                                        | $\lambda$                                                                             | $\eta$                                        | $K$   |
|-----|-----------------------------------------------|-----------------------------------------------------------------------------------------------|---------------------------------------------------------------------------------------|-----------------------------------------------|-------|
| 0.7 | $\begin{bmatrix} 1/2 & 0 & 1/2 \end{bmatrix}$ | $\begin{bmatrix} 1/3 & 1/3 & 1/3 & 0 \\ 1 & 0 & 0 & 0 \\ 1/4 & 1/4 & 1/4 & 1/4 \end{bmatrix}$ | $\begin{bmatrix} 1/3 & 1/3 & 1/3 \\ 1/3 & 1/3 & 1/3 \\ 1/3 & 1/3 & 1/3 \end{bmatrix}$ | $\begin{bmatrix} 1/2 & 1/2 & 0 \end{bmatrix}$ | 'all' |

**Table S8.** Parameters of the RWR for the universal multilayer network used to train and test the classifier. Top: parameters for the multilayer network composed of the gene multiplex network and disease monoplex network (2-multiplex network). Bottom: parameters for the multilayer network composed of the gene, drug multiplex networks, and disease monoplex network (3-multiplex network).

### C.2. Comparative analysis of the results obtained from multilayer networks composed of two or three multiplex networks.

We have seen before more is not always better, it depends on the quality of the bipartite networks and the compatibility between the data of each multiplex network. So adding new data is a delicate task. The LOOCV/LP gives us a way to determine if adding new multiplex networks is better or worst than adding random networks (see section 4.A.4), it is a good way to know if more signal than noise is added. Furthermore, the exploration of the parameter space gives us a method to determine if the scores are stable under input parameters changes.

However it still a question regarding the adding of a new multiplex network in the bring of qualitative information, for example even if quantitatively in the LOOCV/LP the results are not better, i.e no more associations are predicted, maybe the associations predict can be more informative. To test this we use the previous machine learning process described in Fig. S19, to determine if the prediction is better when we using output scores from three multiplex networks than when we using output scores from two multiplex networks. The biological networks is described previously in the section 3.B.

For both multilayer networks, one is composed of a gene multiplex network and a disease monoplex network, and one other is composed of genes and drug multiplex networks and a disease monoplex network. We use the best random forest classifier (highlighted in orange in both tables S9 and S10), extracted from the comparison Table S9 and Table S10, this classifier are trained and tested according to the previous process with different parameters of classifier. The result shows that the multilayer network composed of three multiplex networks do not increase the predictive power of the classifier, worst, it decreases the performance (F1 score in the table S9 and S10). This result rejoins the previous results with the LOOCV/LP protocol, where if the bipartite networks are not adapted to the whole multilayer, more is not better. Hence the necessity to associated with MultiXrank protocols to determine signal-to-noise ratio, exploration of the stability, and alternative way to exploit universal multilayer networks.

| model classifier                                  | Y == 0 | Y == 1 | Y       | F1 score | weights            |
|---------------------------------------------------|--------|--------|---------|----------|--------------------|
| Random Forest (100 estimators)                    | 88,28% | 35,54% | 61,91%  | 0,4827   | none               |
| Random Forest (200 estimators)                    | 90,80% | 30,56% | 60,68%  | 0,4373   | none               |
| Random Forest (1000 estimators)                   | 90,93% | 31,57% | 61,25%  | 0,4489   | none               |
| Gradient Boosting                                 | 80,40% | 49,91% | 65,15%  | 0,5888   | none               |
| Decision Tree weight 0                            | 89,60% | 25,52% | 57,56%  | 0,3755   | 0 : 0.1, 1 : 0.9   |
| Decision Tree weight 1                            | 77,63% | 31,82% | 54,73%  | 0,4128   | 0 : 0.2, 1 : 0.8   |
| Decision Tree weight 2                            | 81,10% | 29,24% | 55,17%  | 0,3947   | 0 : 0.3, 1 : 0.7   |
| Decision Tree weight 3                            | 81,73% | 20,29% | 51,01%  | 0,2929   | 0 : 0.4, 1 : 0.6   |
| Decision Tree weight 4                            | 67,55% | 58,29% | 62,92%  | 0,6112   | 0 : 0.5, 1 : 0.5   |
| Decision Tree weight 5                            | 63,96% | 59,80% | 61,88%  | 0,6107   | 0 : 0.6, 1 : 0.4   |
| Decision Tree weight 6                            | 65,60% | 42,28% | 53,94%  | 0,4786   | 0 : 0.7, 1 : 0.3   |
| Decision Tree weight 7                            | 25,33% | 75,24% | 50,28%  | 0,6021   | 0 : 0.8, 1 : 0.2   |
| Decision Tree weight 8                            | 12,98% | 81,29% | 47,13%  | 0,6059   | 0 : 0.9, 1 : 0.1   |
| Random Forest (100 estimators) 0                  | 99,05% | 2,02%  | 50,54%  | 0,0392   | 0 : 0.1, 1 : 0.9   |
| Random Forest (100 estimators) 1                  | 96,66% | 8,88%  | 52,77%  | 0,1583   | 0 : 0.2, 1 : 0.8   |
| Random Forest (100 estimators) 2                  | 96,16% | 10,84% | 53,50%  | 0,1890   | 0 : 0.3, 1 : 0.7   |
| Random Forest (100 estimators) 3                  | 91,43% | 26,97% | 59,20%  | 0,3980   | 0 : 0.4, 1 : 0.6   |
| Random Forest (100 estimators) 4                  | 88,97% | 38,44% | 63,71%  | 0,5143   | 0 : 0.5, 1 : 0.5   |
| Random Forest (100 estimators) 5                  | 83,55% | 48,96% | 66,26%  | 0,5920   | 0 : 0.6, 1 : 0.4   |
| Random Forest (100 estimators) 6                  | 68,43% | 73,53% | 70,98%  | 0,7171   | 0 : 0.7, 1 : 0.3   |
| Random Forest(100 estimators) 7                   | 36,80% | 93,57% | 65,19%  | 0,7288   | 0 : 0.8, 1 : 0.2   |
| Random Forest (100 estimators) 8                  | 13,36% | 99,24% | 56,30 % | 0,6943   | 0 : 0.9, 1 : 0.1   |
| Random Forest (1000 estimators) 6                 | 93,01% | 87,78% | 90,39%  | 0,9013   | 0 : 0.7, 1 : 0.3   |
| Random Forest (100 estimators) balanced           | 90,42% | 31,19% | 60,81%  | 0,4432   | balanced           |
| Random Forest (100 estimators) balanced subsample | 90,04% | 31,88% | 60,96%  | 0,4496   | balanced subsample |

**Table S9.** Different models of binary classifiers and their accuracies. There are trained and tested according to the process described in Fig. S19. Here we display the results for the multilayer network composed of a gene multiplex network and the disease monoplex network. The classifier highlighted in orange is the most accurate, because it offers high F1 score with balance predictions for the associations labeled 0 or 1. The classifier highlighted in yellow is a good alternative classifier. For each classifier: the columns Y==0, Y==1, displays the percentage of negative (Y==0) and positive (Y==1) gene-disease associations correctly predicted by the classifier, the column Y is the percentage of gene-disease associations correctly predicted by the classifier, and the two last columns display the F1 score and the weights chosen for each class of the classifier.

| model classifier                 | Y == 0  | Y == 1  | Y       | F1 score | weights          |
|----------------------------------|---------|---------|---------|----------|------------------|
| Random Forest (100 estimators) 0 | 91,05 % | 16,26 % | 53,65 % | 0,2597   | 0 : 0,1, 1 : 0,9 |
| Random Forest (100 estimators) 1 | 89,41 % | 19,28 % | 54,35 % | 0,2969   | 0 : 0,2, 1 : 0,8 |
| Random Forest (100 estimators) 2 | 88,78 % | 19,47 % | 54,13 % | 0,2980   | 0 : 0,3, 1 : 0,7 |
| Random Forest (100 estimators) 3 | 88,15 % | 21,80 % | 54,98 % | 0,3263   | 0 : 0,4, 1 : 0,6 |
| Random Forest (100 estimators) 4 | 85,32 % | 22,94 % | 54,13 % | 0,3333   | 0 : 0,5, 1 : 0,5 |
| Random Forest (100 estimators) 5 | 84,37 % | 26,21 % | 55,29 % | 0,3696   | 0 : 0,6, 1 : 0,4 |
| Random Forest (100 estimators) 6 | 80,91 % | 30,81 % | 55,86 % | 0,4111   | 0 : 0,7, 1 : 0,3 |
| Random Forest(100 estimators) 7  | 74,10 % | 35,54 % | 54,82 % | 0,4403   | 0 : 0,8, 1 : 0,2 |
| Random Forest (100 estimators) 8 | 60,49 % | 64,27 % | 62,38 % | 0,6308   | 0 : 0,9, 1 : 0,1 |

**Table S10.** Different models of binary classifiers and their accuracies. There are training and testing according to the process described in Fig. S19. Here we display the results for the multilayer network composed of genes, drug multiplex networks and a disease monoplex network. The classifier highlighted in orange is the most accurate, because it offers high F1 score with balance predictions for the associations labeled 0 or 1. For each classifier: the columns Y==0, Y==1, displays the percentage of negative (Y==0) and positive (Y==1) gene-disease associations correctly predicted by the classifier, the column Y is the percentage of gene-disease associations correctly predicted by the classifier, and the two last columns display the F1 score and the weights chosen for each class of the classifier.

## References

1. Valdeolivas A, et al. (2018) Random walk with restart on multiplex and heterogeneous biological networks. *Bioinformatics* 35(3):497–505.
2. Li Y, Patra JC (2010) Genome-wide inferring gene–phenotype relationship by walking on the heterogeneous network. *Bioinformatics* 26(9):1219–1224.
3. Jin W, Jung J, Kang U (2019) Supervised and extended restart in random walks for ranking and link prediction in networks. *PLOS ONE* 14(3):e0213857.
4. Cardillo A, et al. (2013) Emergence of network features from multiplexity. *Scientific Reports* 3(1):1344.
5. Drew K, et al. (2017) Integration of over 9,000 mass spectrometry experiments builds a global map of human protein complexes. *Mol Syst Biol* 13(6):932.
6. Giurgiu M, et al. (2019) Corum: the comprehensive resource of mammalian protein complexes–2019. *Nucleic Acids Res* 47(D1):D559–D563.
7. Türe D, et al. (2020) Integrated intra- and intercellular signaling knowledge for multicellular omics analysis. *bioRxiv* p. 2020.08.03.221242.
8. Pratt D, et al. (2015) Ndex, the network data exchange. *Cell Systems* 1(4):302–305.
9. Croft D, et al. (2014) The reactome pathway knowledgebase. *Nucleic Acids Res* 42(D1):D472–D477.
10. Cheng F, Kovács IA, Barabási AL (2019) Network-based prediction of drug combinations. *Nature Communications* 10(1):1197.
11. Piñero J, et al. (2020) The disgenet knowledge platform for disease genomics: 2019 update. *Nucleic Acids Res* 48(D1):D845–D855.
12. Brown AS, Patel CJ (2017) A standard database for drug repositioning. *Scientific Data* 4(1):170029.
13. Himmelstein DS, et al. (2017) Systematic integration of biomedical knowledge prioritizes drugs for repurposing. *eLife* 6:e26726.
14. Mordelet F, Vert JP (2011) Prodiges: Prioritization of disease genes with multitask machine learning from positive and unlabeled examples. *BMC Bioinformatics* 12(1):389.
15. Tyner JW, et al. (2009) High-throughput sequencing screen reveals novel, transforming ras mutations in myeloid leukemia patients. *Blood* 113(19075190):1749–1755.
16. Thomas X, Elhamri M (2007) Tipifarnib in the treatment of acute myeloid leukemia. *Biologics : targets & therapy* 1(19707311):415–424.
17. Karp JE, Lancet JE (2008) Tipifarnib in the treatment of newly diagnosed acute myelogenous leukemia. *Biologics : targets & therapy* 2(3):491–500.
18. Yanamandra N, et al. (2011) Tipifarnib-induced apoptosis in acute myeloid leukemia and multiple myeloma cells depends on  $Ca^{2+}$  influx through plasma membrane  $Ca^{2+}$  channels. *J Pharmacol Exp Ther* 337(3):636.
19. Runtz L, et al. (2018) Hepatic and hippocampal cytochrome p450 enzyme overexpression during spontaneous recurrent seizures. *Epilepsia* 59(1):123–134.
20. Tomić M, Pecikoza U, Micov A, Vučković S, Stepanović-Petrović R (2018) Antiepileptic drugs as analgesics/adjuvants in inflammatory pain: current preclinical evidence. *Pharmacology & therapeutics* 192:42–64.
21. Swathi K, Sarangapani M (2017) Evaluation of anti-epileptic effect of new indole derivatives by estimation of biogenic amines concentrations in rat brain. *Advances in experimental medicine and biology* 988:39–48.
22. Liu H, et al. (2019) Predicting effective drug combinations using gradient tree boosting based on features extracted from drug-protein heterogeneous network. *BMC Bioinformatics* 20(1):645.
